# Supplementary material for: Correcting Spectra Outside the Backbone: A Model-Agnostic Rectifier for Hyperspectral Image Super-Resolution
Source: arXiv:2601.21338 source file (2026-09-28)
Supplement: Supplementary file 2 [file append.tex]

\section{Method}
\subsection{H-S$^{3}$A: Cross-Band Interaction Enhancement}
\paragraph{Convolutions after spectral grouping.}
After spectral grouping, we apply a lightweight convolutional stem \emph{within each group} before entering TSA.
Specifically, each group is processed by a set of convolutions with complementary receptive fields, including a identity, a standard $3\times3$ convolution, a $5\times5$ depthwise convolution, and a $3\times3$ dilated convolution, followed by a $1\times1$ convolution for channel mixing and projection.

% This design enriches local spectral--spatial cues at multiple effective receptive fields while keeping the computation efficient.
% The resulting per-group features are then fed into TSA for cross-group interaction; the outputs from all groups are concatenated and fused by a final $1\times1$ convolution to form the rectified representation.

\paragraph{Handling non-divisible channel grouping in H-S$^{3}$A.}
H-S$^{3}$A performs group-wise spectral processing, which requires the spectral channel number to be divisible by the group size.
When this condition is not met, we pad the input along the channel dimension with additional channels so that the padded channel number becomes divisible by the number of groups.

\subsection{Manifold-Consistency Rectification Details}
The MCR module consists of three key components, namely the \textit{Manifold Block}, \textit{Refine Block}, and \textit{Back-Block}.

The \textit{Manifold Block} is designed to project high-dimensional spectral features onto a low-dimensional manifold. It is composed of a $1\times1$ convolution followed by a GeLU activation function, where the $1\times1$ convolution reduces the channel dimension from $C$ to $r$.

The \textit{Refine Block} operates in the manifold space to progressively refine the embedded features. It shares a similar structure with the Manifold Block, consisting of a $1\times1$ convolution and a GeLU activation function, while keeping the channel dimension unchanged at $r$.

The \textit{Back-Block} maps the refined manifold features back to the original spectral space and generates the corresponding rectification components. It comprises a $3\times3$ convolution, a GeLU activation function, and a $1\times1$ convolution, and adopts a residual formulation. The computation can be expressed as
\begin{equation}
f_{\text{output}} = \mathrm{Conv}_{1\times1}\!\left(
\mathrm{GeLU}\!\left(\mathrm{Conv}_{3\times3}(f_{\text{input}})\right)
+ f_{\text{input}}
\right),
\end{equation}
where the final $1\times1$ convolution expands the channel dimension from $r$ back to $C$.
%
% The padded channels are treated as regular channels and participate in all intermediate computations, ensuring that tensor shapes remain consistent throughout the group-wise operations.
% After the final projection (the last $1\times1$ convolution), we remove the padded channels and restore the original channel number, so that the module preserves the input--output tensor shape.

\section{Experiments}

\subsection{Full Error Map Gallery}

We provide representative error-map visualizations on ARAD-1K, CAVE, and ICVL to complement the quantitative results, as shown in Figs.~\ref{fig:errmap_arad}--\ref{fig:errmap_icvl}.
Each page contains two test scenes. For each scene, we show the pseudo-RGB rendering and the corresponding error maps of different SR backbones, where the rectified variant is placed next to its baseline for direct comparison.

Given a reconstructed HSI $\hat{\mathbf{I}}_{\mathrm{HR}}$ and the ground truth $\mathbf{I}_{\mathrm{HR}}$ with $S=31$ spectral bands,
we compute a per-pixel error map by averaging the absolute reconstruction error across bands:
\begin{equation}
E(i,j)=\frac{1}{S}\sum_{s=1}^{S}\left|\hat{\mathbf{I}}_{\mathrm{HR}}(i,j,s)-\mathbf{I}_{\mathrm{HR}}(i,j,s)\right|.
\end{equation}
For consistent display, we apply per-image min--max normalization and obtain $\tilde{E}\in[0,1]$:
\begin{equation}
\tilde{E}=\frac{E-\min(E)}{\max(E)-\min(E)},
\end{equation}
where $\min(\cdot)$ and $\max(\cdot)$ are computed over all pixels within the same image.
Pseudo-RGB images are rendered by mapping bands $25$, $15$, and $5$ to the red, green and blue channels, followed by the same linear min--max stretch and clipping to $[0,1]$ for all methods.

As illustrated in Figs.~\ref{fig:errmap_arad}--\ref{fig:errmap_icvl}, darker regions indicate smaller reconstruction error, while brighter regions highlight locations where the reconstruction deviates from the ground truth.
Across datasets, the dominant errors of baseline models typically concentrate on object boundaries, thin structures, and high-frequency textures, where cross-band inconsistency is more likely to appear as visible artifacts.
By placing the rectified outputs next to the corresponding baselines, the gallery highlights that~\name mainly suppresses boundary-related errors without washing out fine details.

\subsection{Additional Spectral Curve Visualizations}

We provide additional per-pixel spectral curve visualizations on ARAD-1K, CAVE, and ICVL to complement the quantitative comparisons and the spectral example in the main paper, as shown in Figs.~\ref{fig:sp_arad_gallery}--\ref{fig:sp_icvl_gallery}.
Each page contains two test scenes. For each scene, we mark two pixels on the pseudo-RGB rendering and plot the spectral signatures over all $31$ bands for the ground truth, the baseline output, and the rectified output obtained by appending~\name.

All results are reported at the $\times4$ scale. Pseudo-RGB images are rendered by mapping bands $25$, $15$, and $5$ to the RGB channels. The plots include CNN-, Transformer-, and Diffusion-based backbones, and DDS2M is visualized together with the other models under the same setting.

Real hyperspectral signatures typically vary smoothly with wavelength. In contrast, baseline SR models may introduce band-to-band oscillations, local spectral shifts, or distorted peak/valley structures at certain pixels. The rectified outputs consistently better follow the ground-truth trend and suppress non-physical oscillations while preserving the overall spectral shape, including the more challenging diffusion-based reconstructions. These observations align with the consistent improvements in spectral fidelity reported in the main paper.

\subsection{Model Complexity Across Backbones and Scales}
\label{sec:app_complexity}

\paragraph{Protocol.}
We report the number of parameters and FLOPs for each SR backbone and its rectified variant (+~\name).
FLOPs are measured on LR inputs of size $64\!\times\!64$ for $\times2$ and $32\!\times\!32$ for $\times4, \times8$,
following the patch sizes used in training.

\begin{table}[htbp]
\centering

\scriptsize
\setlength{\tabcolsep}{3.4pt}

\begin{adjustbox}{min width=\linewidth, max width=\linewidth}
\begin{tabular}{c c|ccc|ccc|ccc|ccc}
\toprule
\multirow{2}{*}{Scale} & \multirow{2}{*}{Metric} &
\multicolumn{3}{c|}{ESSAformer} &
\multicolumn{3}{c|}{RCAN} &
\multicolumn{3}{c|}{SSPSR} &
\multicolumn{3}{c}{SwinIR} \\
& & Base & +Ours & Gain & Base & +Ours & Gain & Base & +Ours & Gain & Base & +Ours & Gain \\
\midrule

\multirow{2}{*}{$\times2$}
& Params (M)
& 8.686  & \ourscell{8.734}  & \gainpos{+0.048}
& 15.479 & \ourscell{15.527} & \gainpos{+0.048}
& 10.534 & \ourscell{10.581} & \gainpos{+0.048}
& 8.080  & \ourscell{8.128}  & \gainpos{+0.048} \\
& FLOPs (G)
& 431.388 & \ourscell{432.871} & \gainpos{+1.482}
& 126.149 & \ourscell{127.632} & \gainpos{+1.482}
& 219.438 & \ourscell{220.920} & \gainpos{+1.482}
& 70.621  & \ourscell{72.104}  & \gainpos{+1.482} \\
\midrule

\multirow{2}{*}{$\times4$}
& Params (M)
& 11.194 & \ourscell{11.242} & \gainpos{+0.048}
& 15.627 & \ourscell{15.675} & \gainpos{+0.048}
& 12.894 & \ourscell{12.942} & \gainpos{+0.048}
& 8.228  & \ourscell{8.276}  & \gainpos{+0.048} \\
& FLOPs (G)
& 409.202 & \ourscell{410.684} & \gainpos{+1.482}
& 33.208  & \ourscell{34.690}  & \gainpos{+1.482}
& 122.200 & \ourscell{123.682} & \gainpos{+1.482}
& 19.302  & \ourscell{20.785}  & \gainpos{+1.482} \\
\midrule

\multirow{2}{*}{$\times8$}
& Params (M)
& 13.702 & \ourscell{13.750} & \gainpos{+0.048}
& 15.774 & \ourscell{15.822} & \gainpos{+0.048}
& 15.254 & \ourscell{15.302} & \gainpos{+0.048}
& 8.376  & \ourscell{8.423}  & \gainpos{+0.048} \\
& FLOPs (G)
& 1614.620 & \ourscell{1620.549} & \gainpos{+5.930}
& 39.889   & \ourscell{45.819}   & \gainpos{+5.930}
& 391.559  & \ourscell{397.488}  & \gainpos{+5.930}
& 25.891   & \ourscell{31.821}   & \gainpos{+5.930} \\
\bottomrule
\end{tabular}
\end{adjustbox}
\caption{Parameters and FLOPs across backbones and scales (ARAD-1K checkpoints).
We report the model size (Params, in millions) and computational cost (FLOPs, in billions).
$\Delta$ denotes the additional cost introduced by~\name.}
\label{tab:app_complexity_all_compact}
\end{table}
\paragraph{Takeaway.}
\name consistently introduces a constant parameter overhead (+0.048M) across backbones.
The FLOPs overhead mainly depends on the HR spatial size: $\times2/\times4$ share the same HR patch size ($128^2$), leading to +1.482G FLOPs, while $\times8$ uses $256^2$, resulting in +5.930G FLOPs.
% =========================
% Appendix D: Degradation mismatch
% (Place after Appendix C)
% =========================
\subsection{Robustness to Test-Time Degradation Mismatch}
\paragraph{Degradation settings.}
All models are trained with the standard synthetic degradation used in the main paper, where the low-resolution input is obtained by bicubic downsampling from the high-resolution hyperspectral image.
We then test robustness under mild mismatch by keeping the trained model fixed and changing the test-time degradation in four ways.
First, we vary the downsampling operator by replacing the training bicubic implementation with either area-based downsampling or an alternative bicubic implementation.
Second, we introduce Gaussian blur in the high-resolution space before downsampling with blur standard deviation $\sigma \in \{0.6, 1.0\}$.
The blur is applied independently to each spectral band using depthwise convolution with reflect padding, and the kernel size follows
$k=\max(3,2\lceil 6\sigma\rceil+1)$, which results in $k=5$ for $\sigma=0.6$ and $k=7$ for $\sigma=1.0$.
Third, we add i.i.d.\ Gaussian noise in the low-resolution space after downsampling with $\epsilon\sim\mathcal{N}(0,\sigma^2)$ and $\sigma=n/255$, where $n\in\{1,2,5\}$.
Finally, we evaluate two combined settings with blur and noise pairs $(\sigma,n)\in\{(0.6,2),(1.0,5)\}$.
For each scale factor, we center-crop high-resolution images so that both spatial dimensions are divisible by the scale.
Noise is generated with a deterministic per-image seed to ensure reproducibility.
Tab.~\ref{tab:app_deg_results_arad_compact} reports the results on ARAD-1K for SwinIR and SwinIR +~\name.
\paragraph{Observation.}
Across all mismatch settings and scales,~\name consistently improves spectral fidelity, as evidenced by lower mSAM.
The advantage becomes more noticeable when the test-time operator deviates from the training downsampling implementation and when blur or noise is present.
At the same time, spatial quality is generally preserved or improved, suggesting that the rectifier mitigates spectral inconsistency without sacrificing spatial reconstruction under mild degradation shifts.

\ErrMapGalleryPage
{Representative error-map gallery on ARAD-1K at $\times4$. For each scene, we show pseudo-RGB renderings and the corresponding band-averaged absolute error maps of different SR backbones, with the rectified result placed next to its baseline for direct comparison.}
{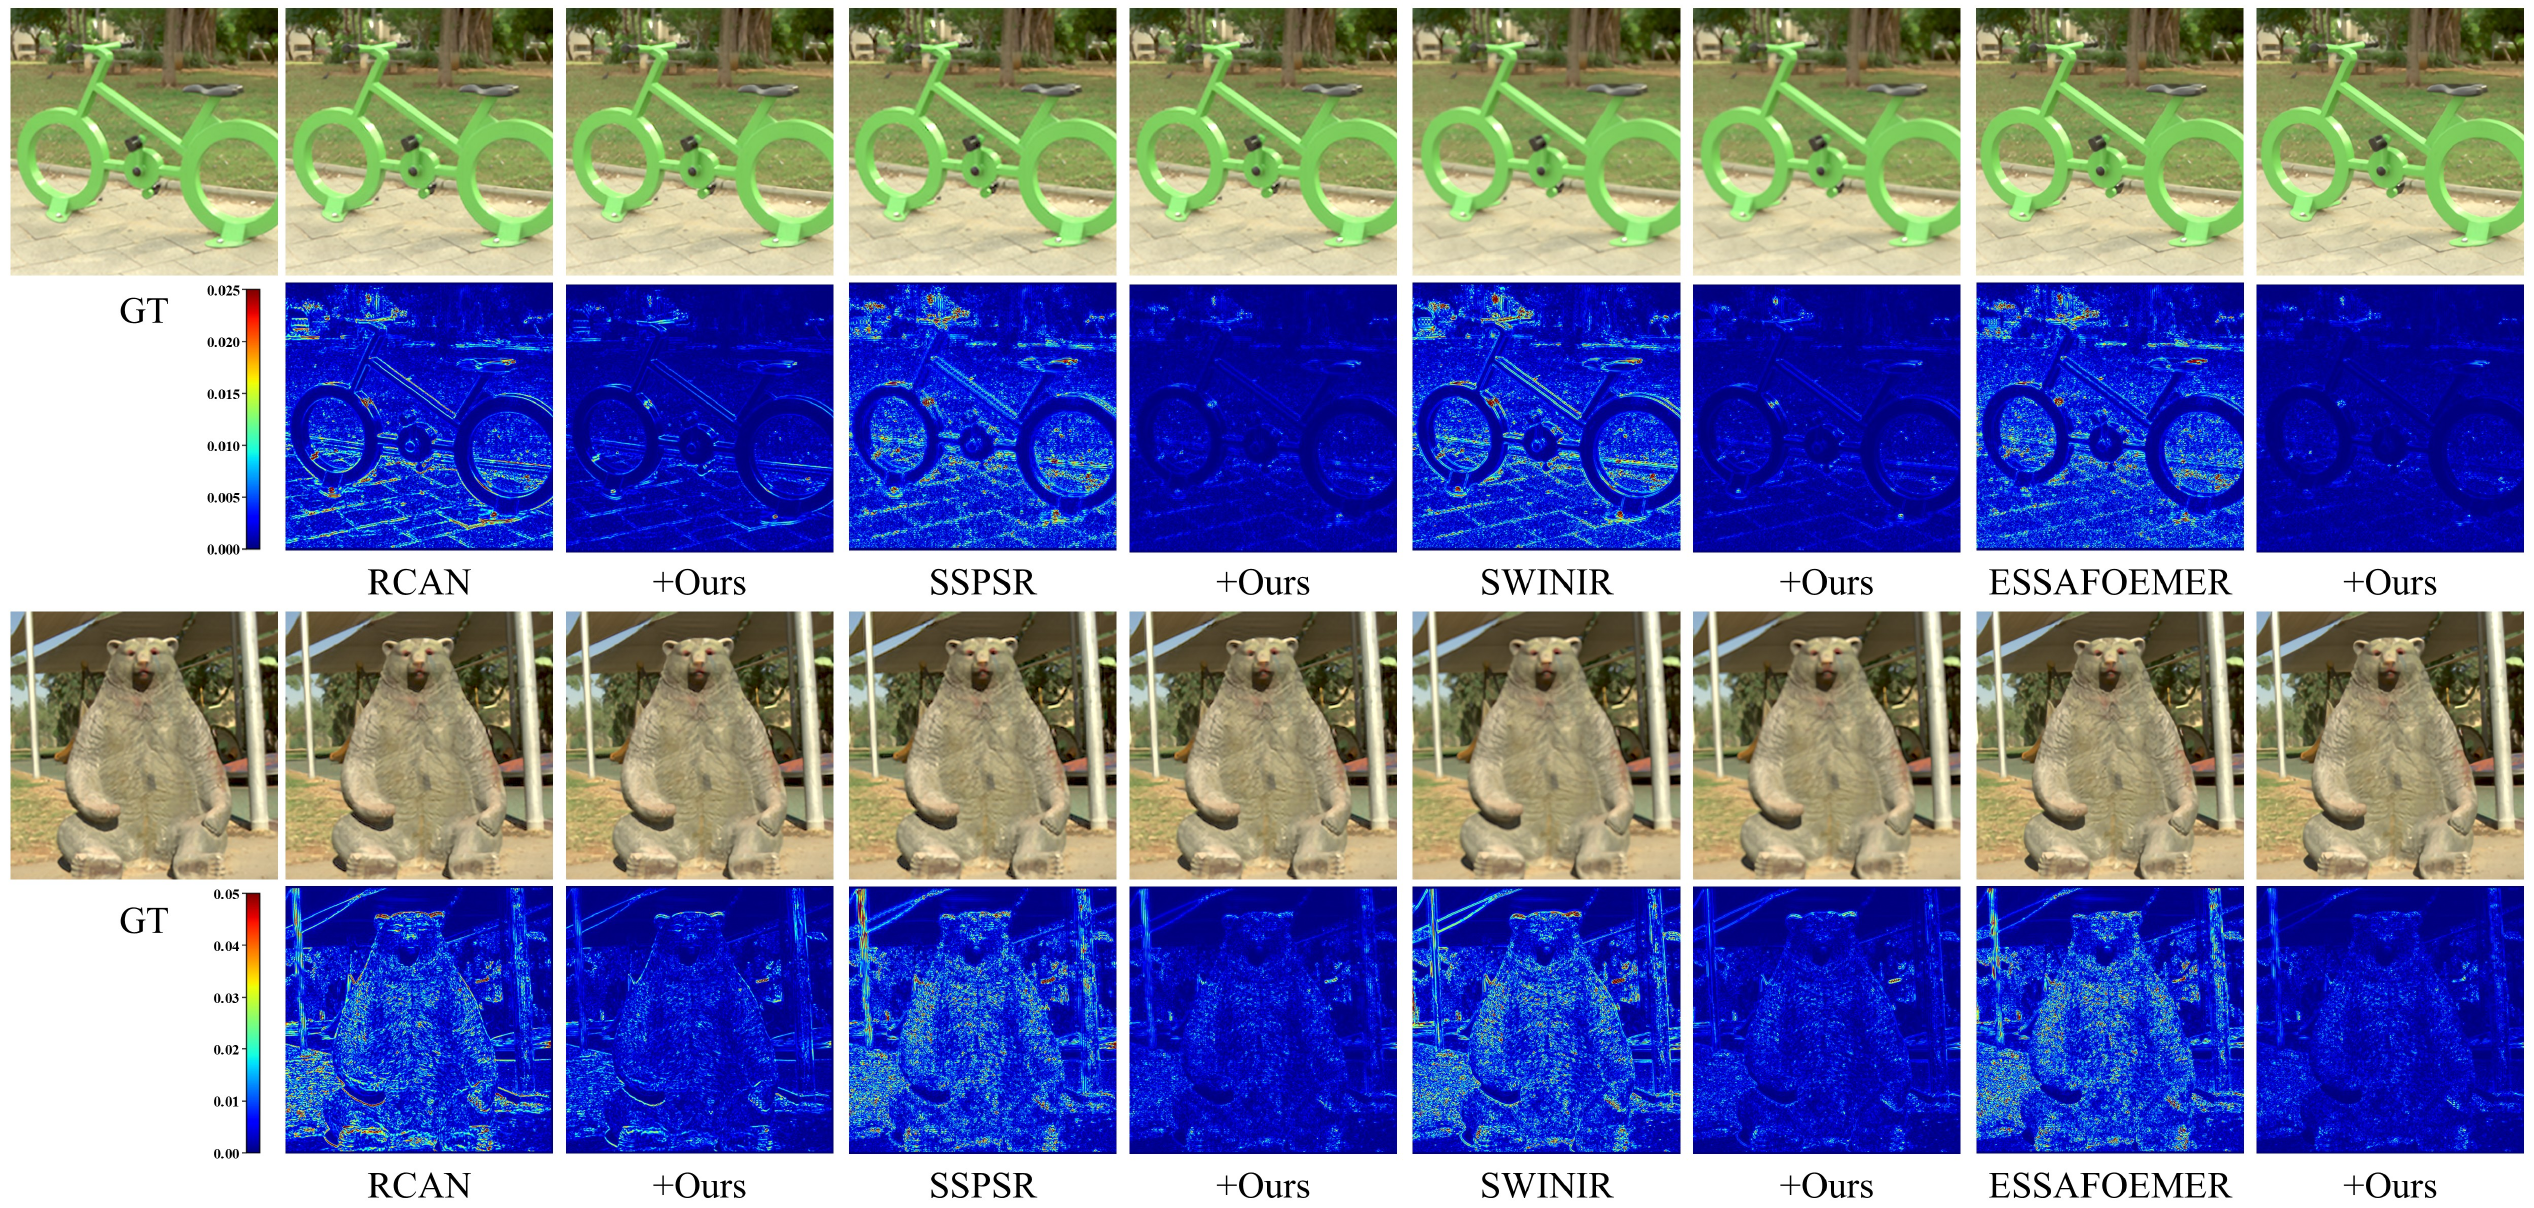}{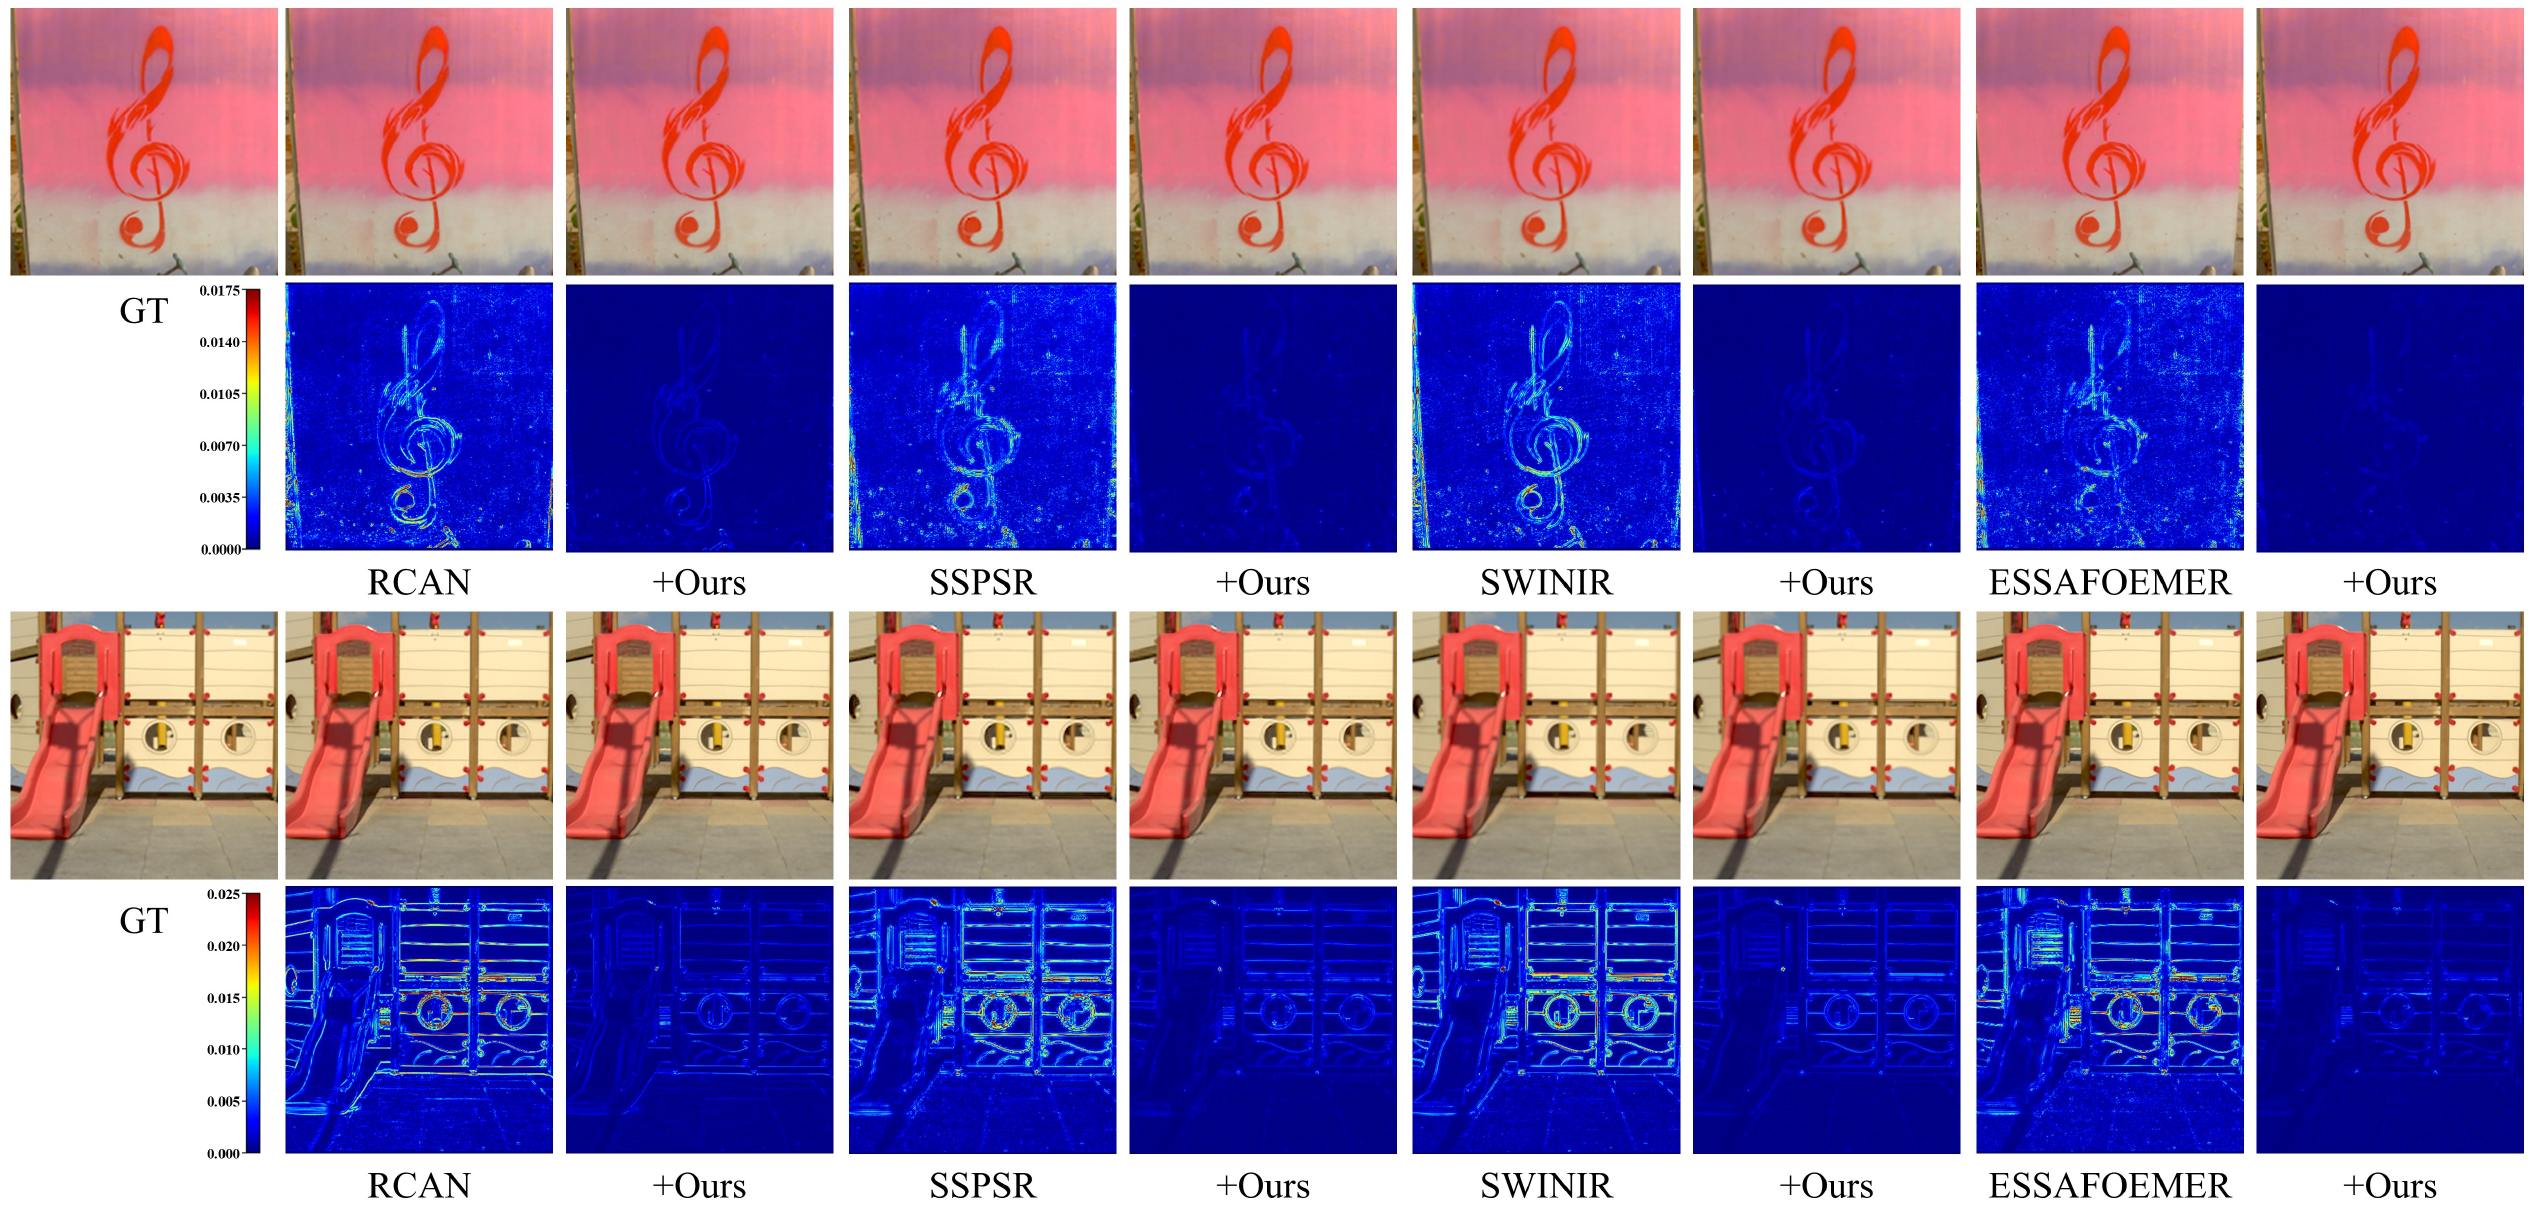}{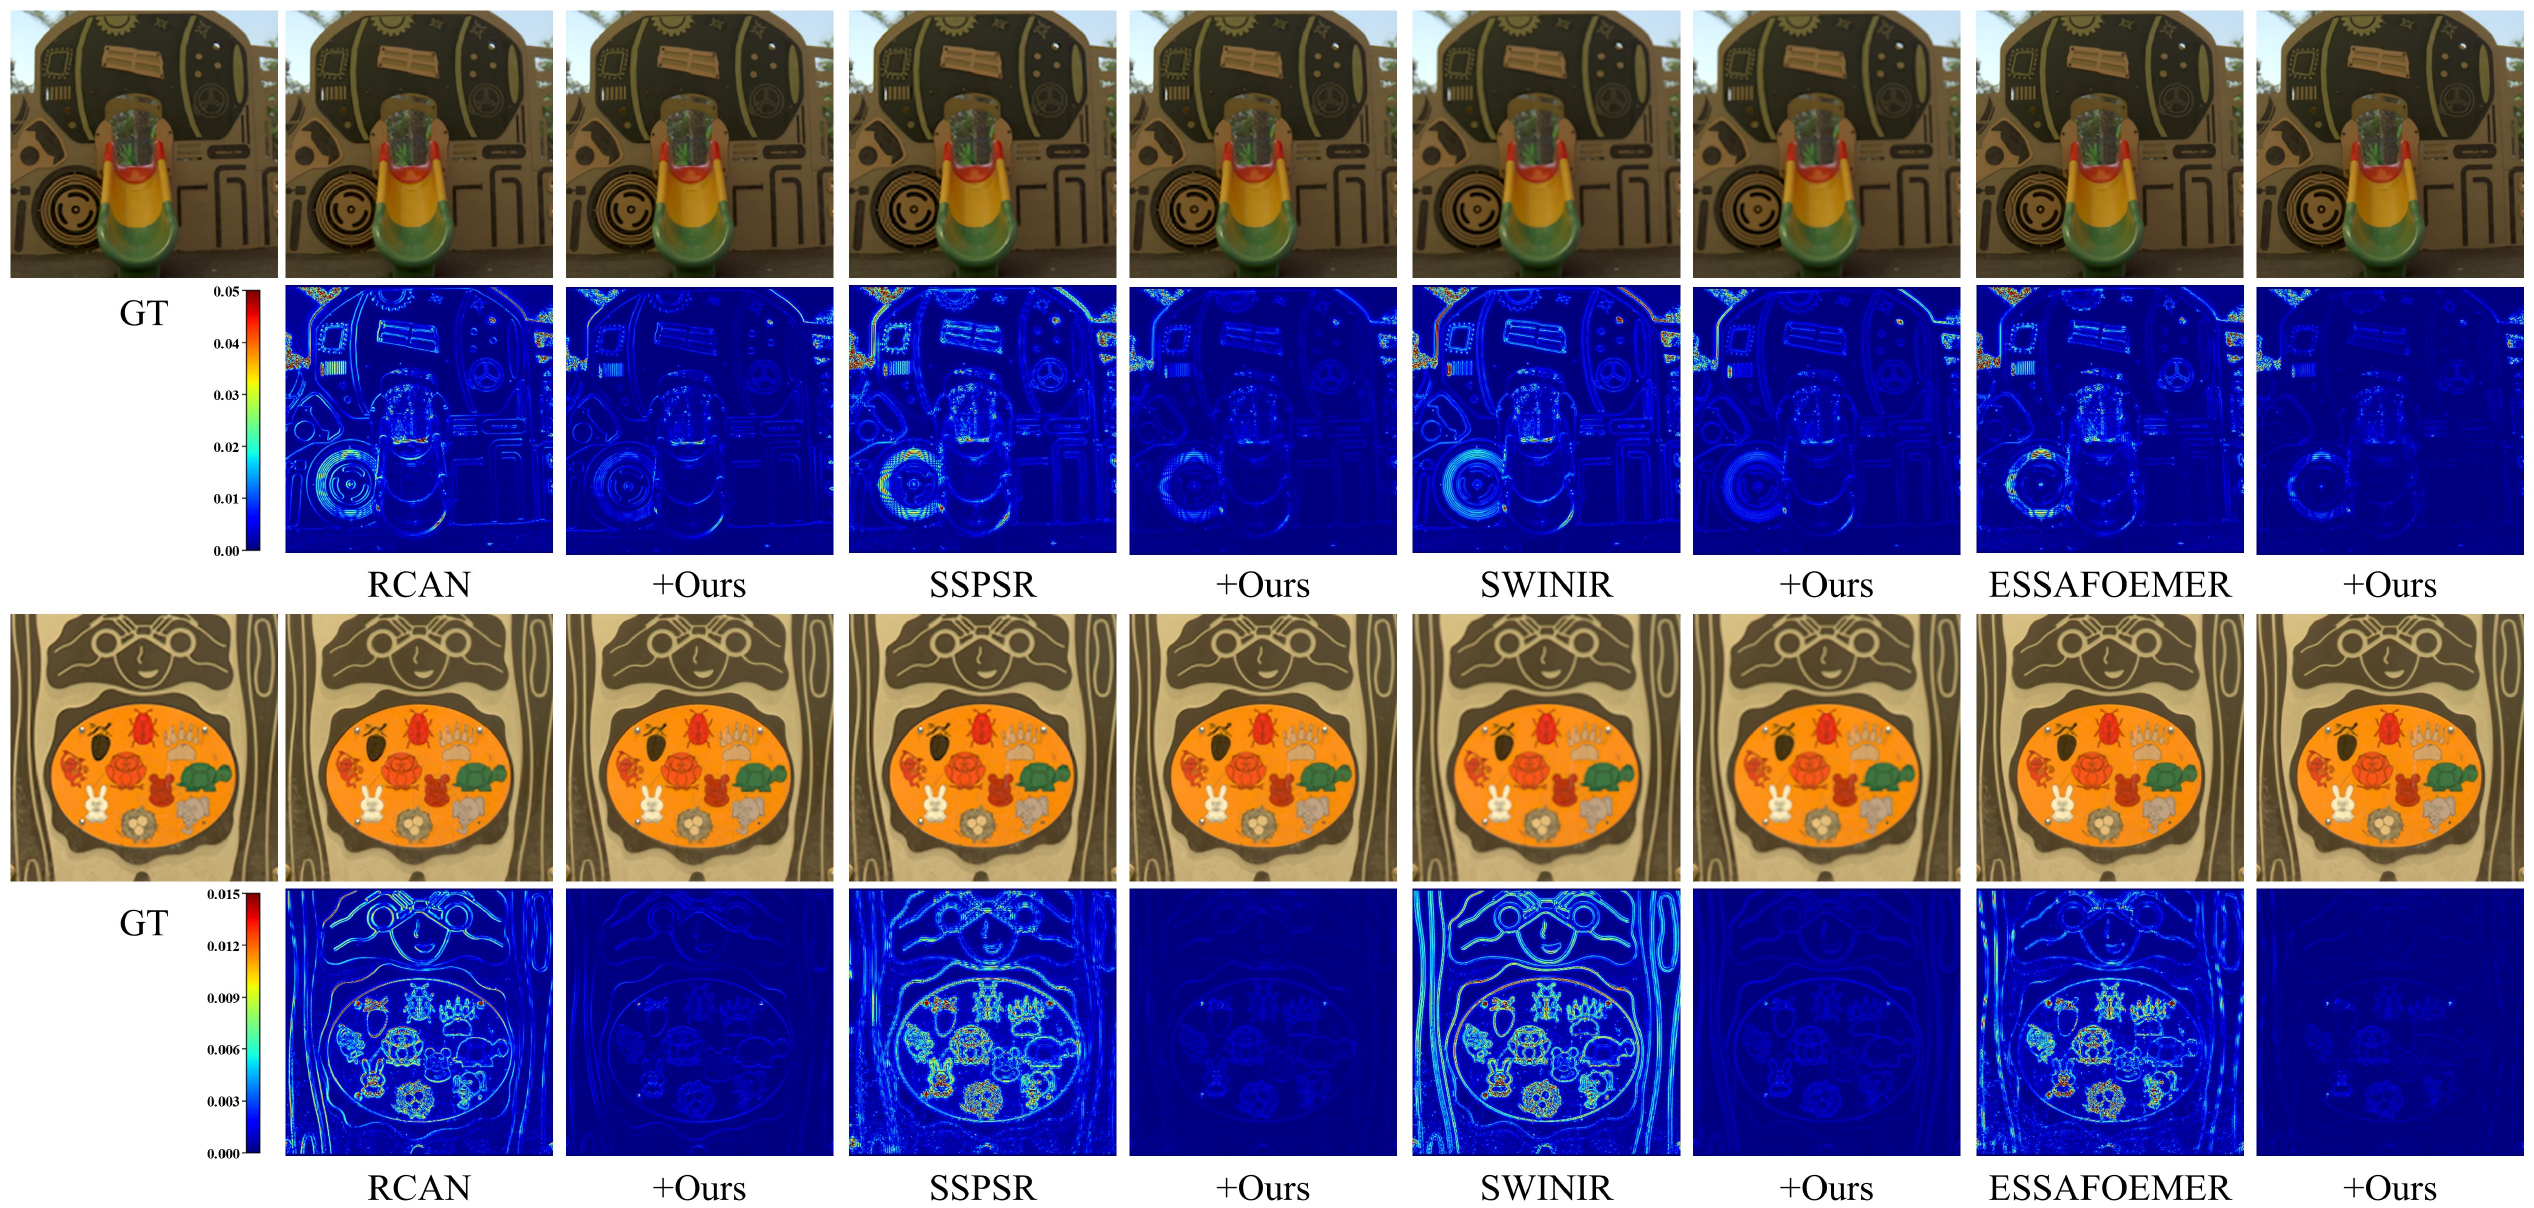}{fig:errmap_arad}

\ErrMapGalleryPage
{Representative error-map gallery on CAVE at $\times4$. The visualization protocol is identical to Fig.~\ref{fig:errmap_arad}.}
{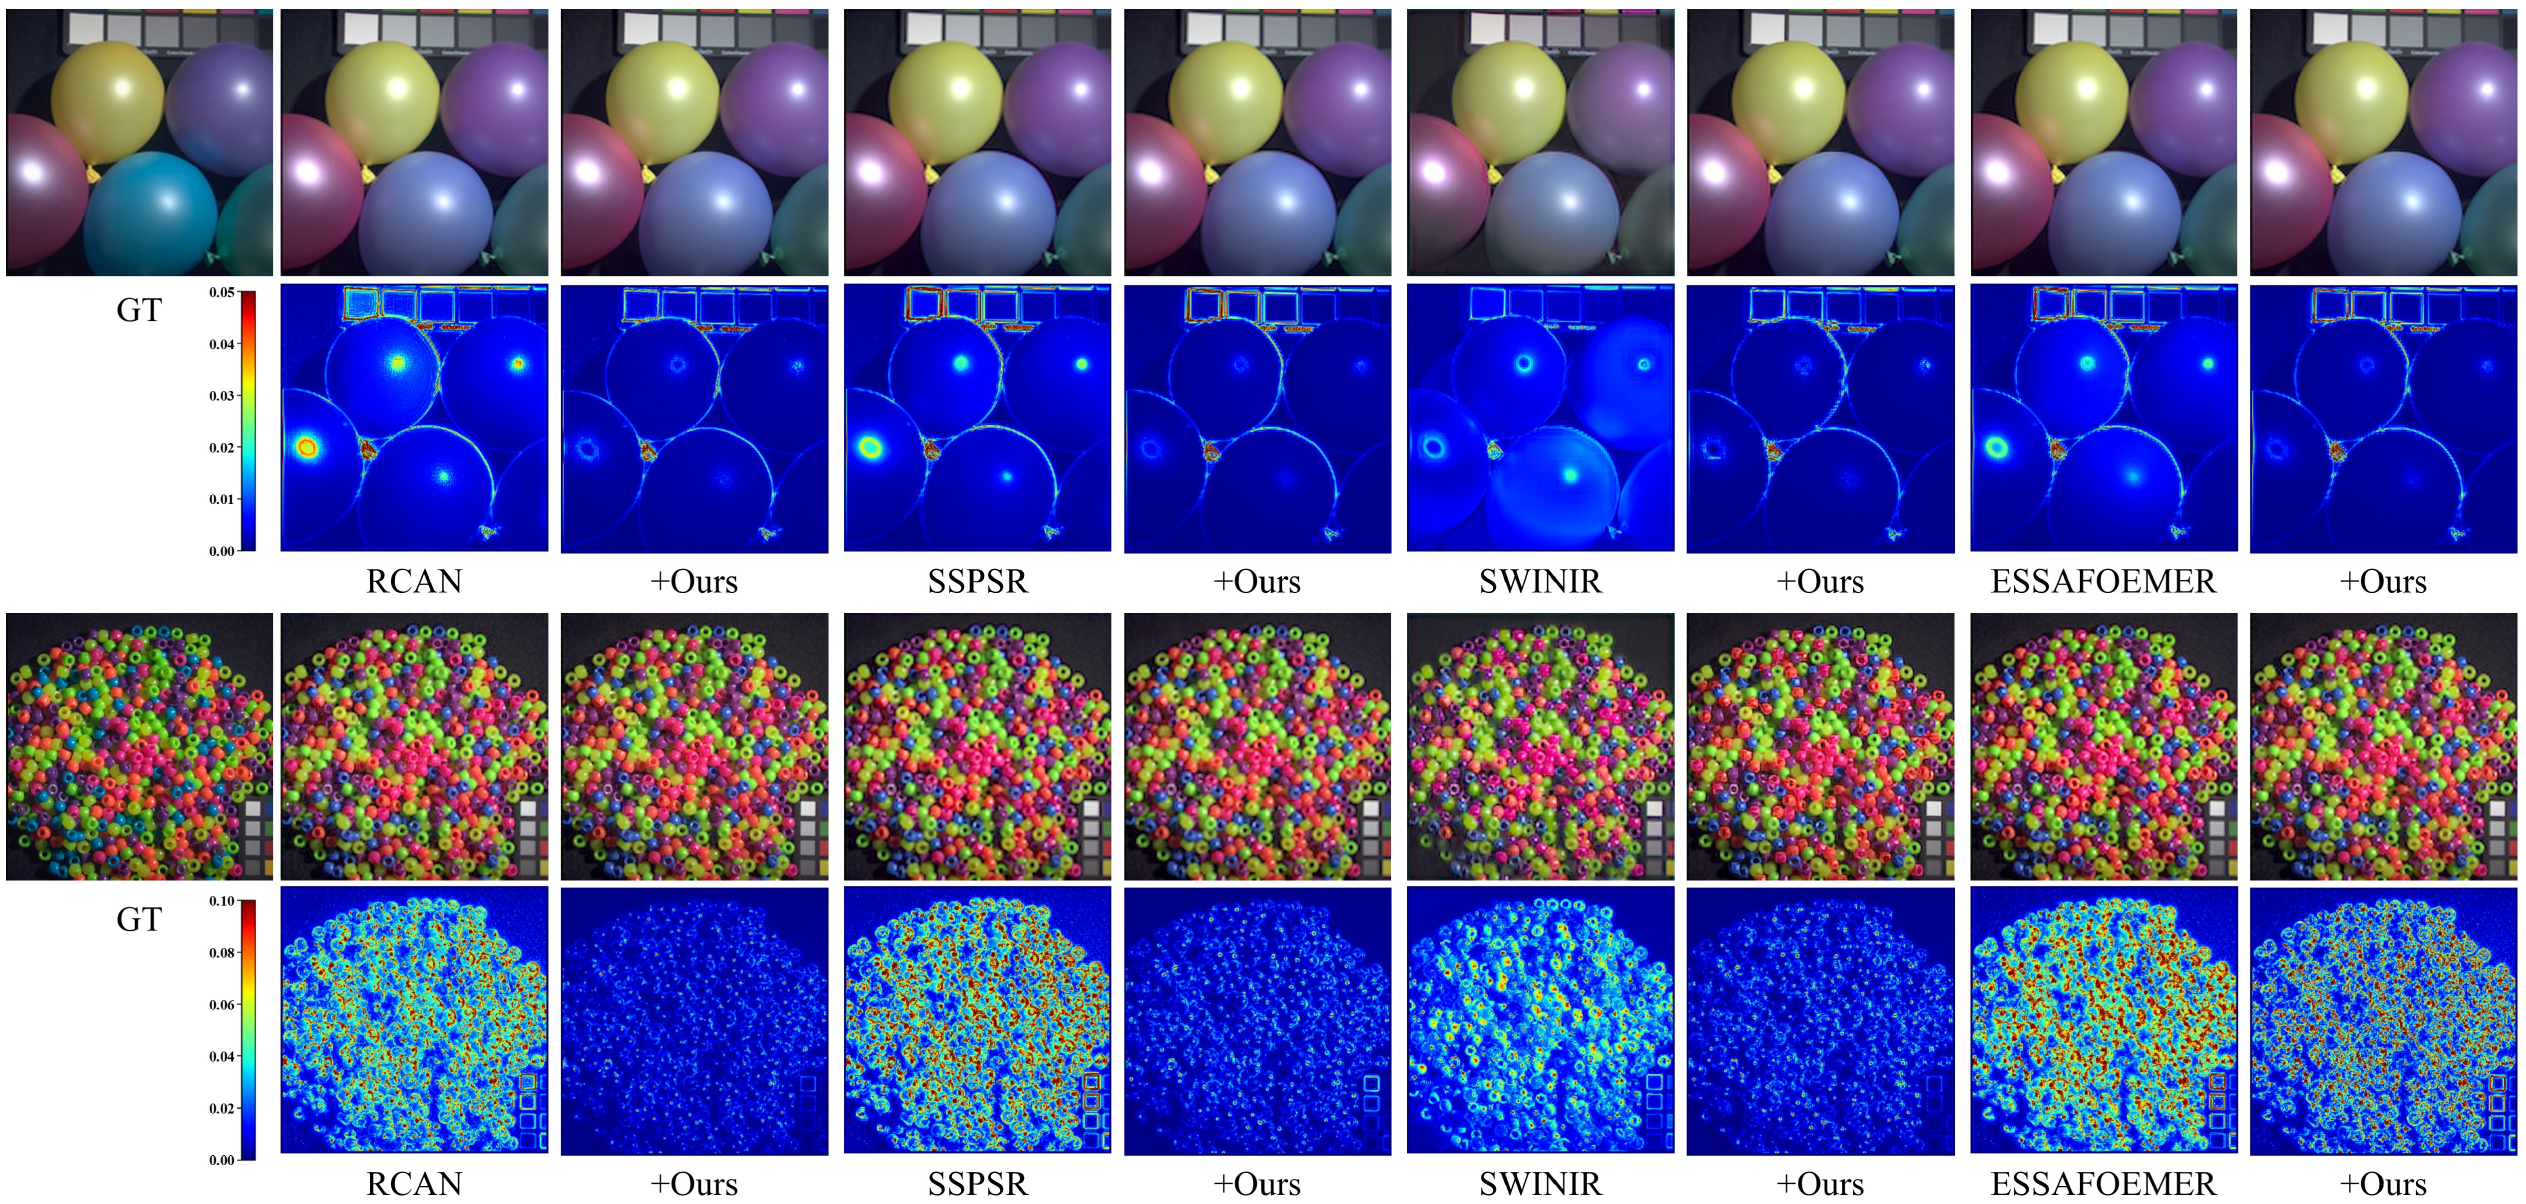}{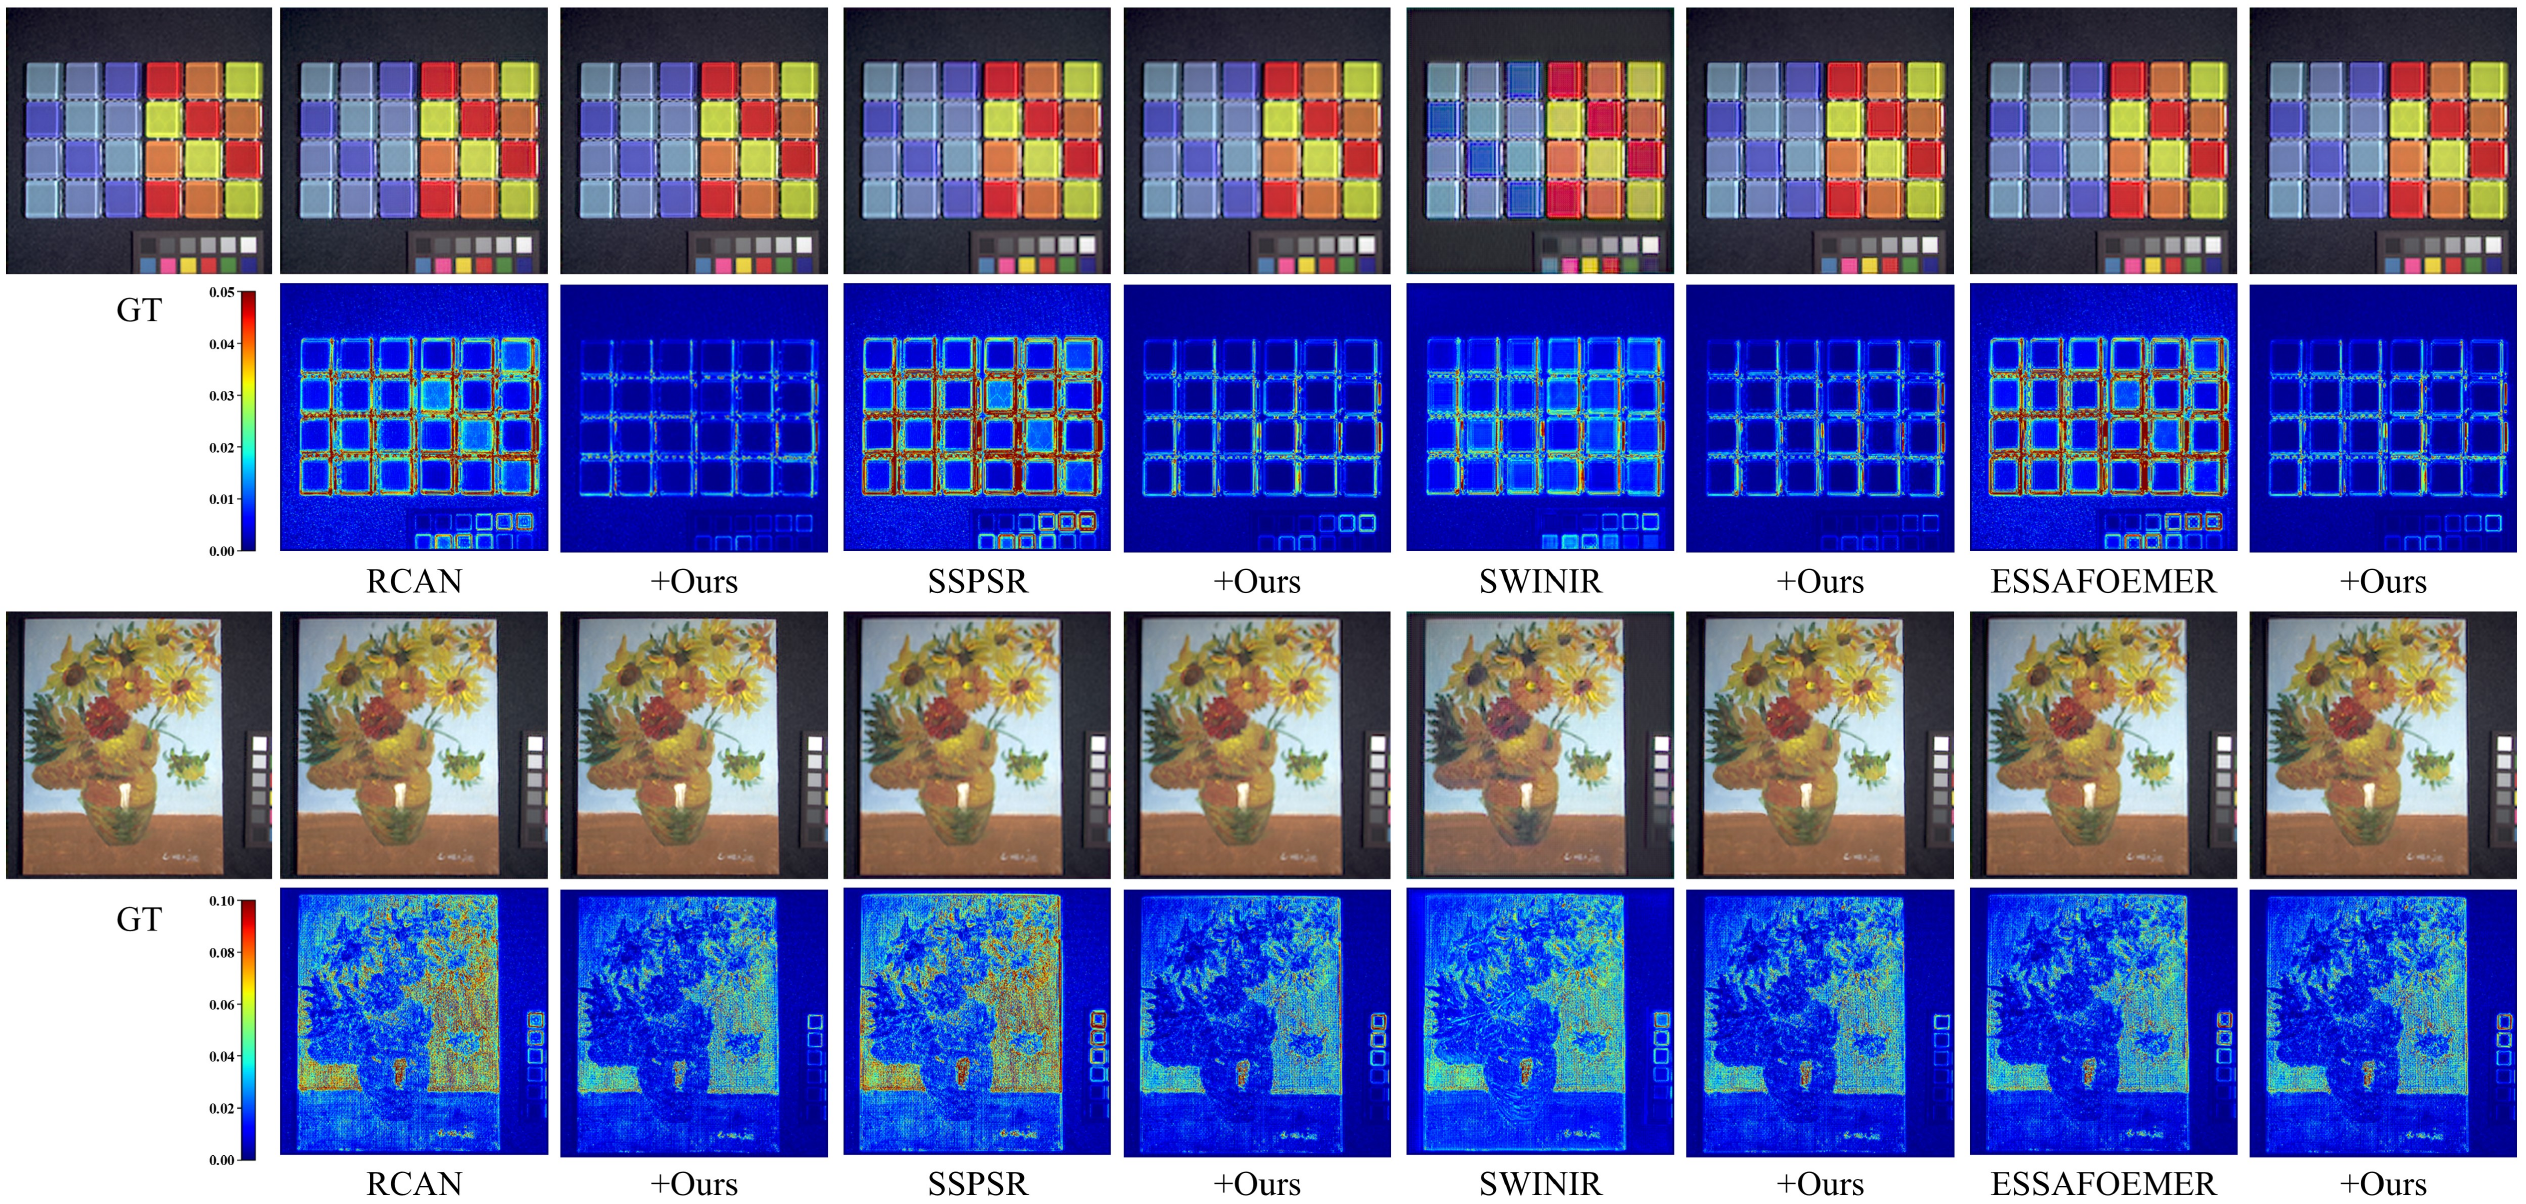}{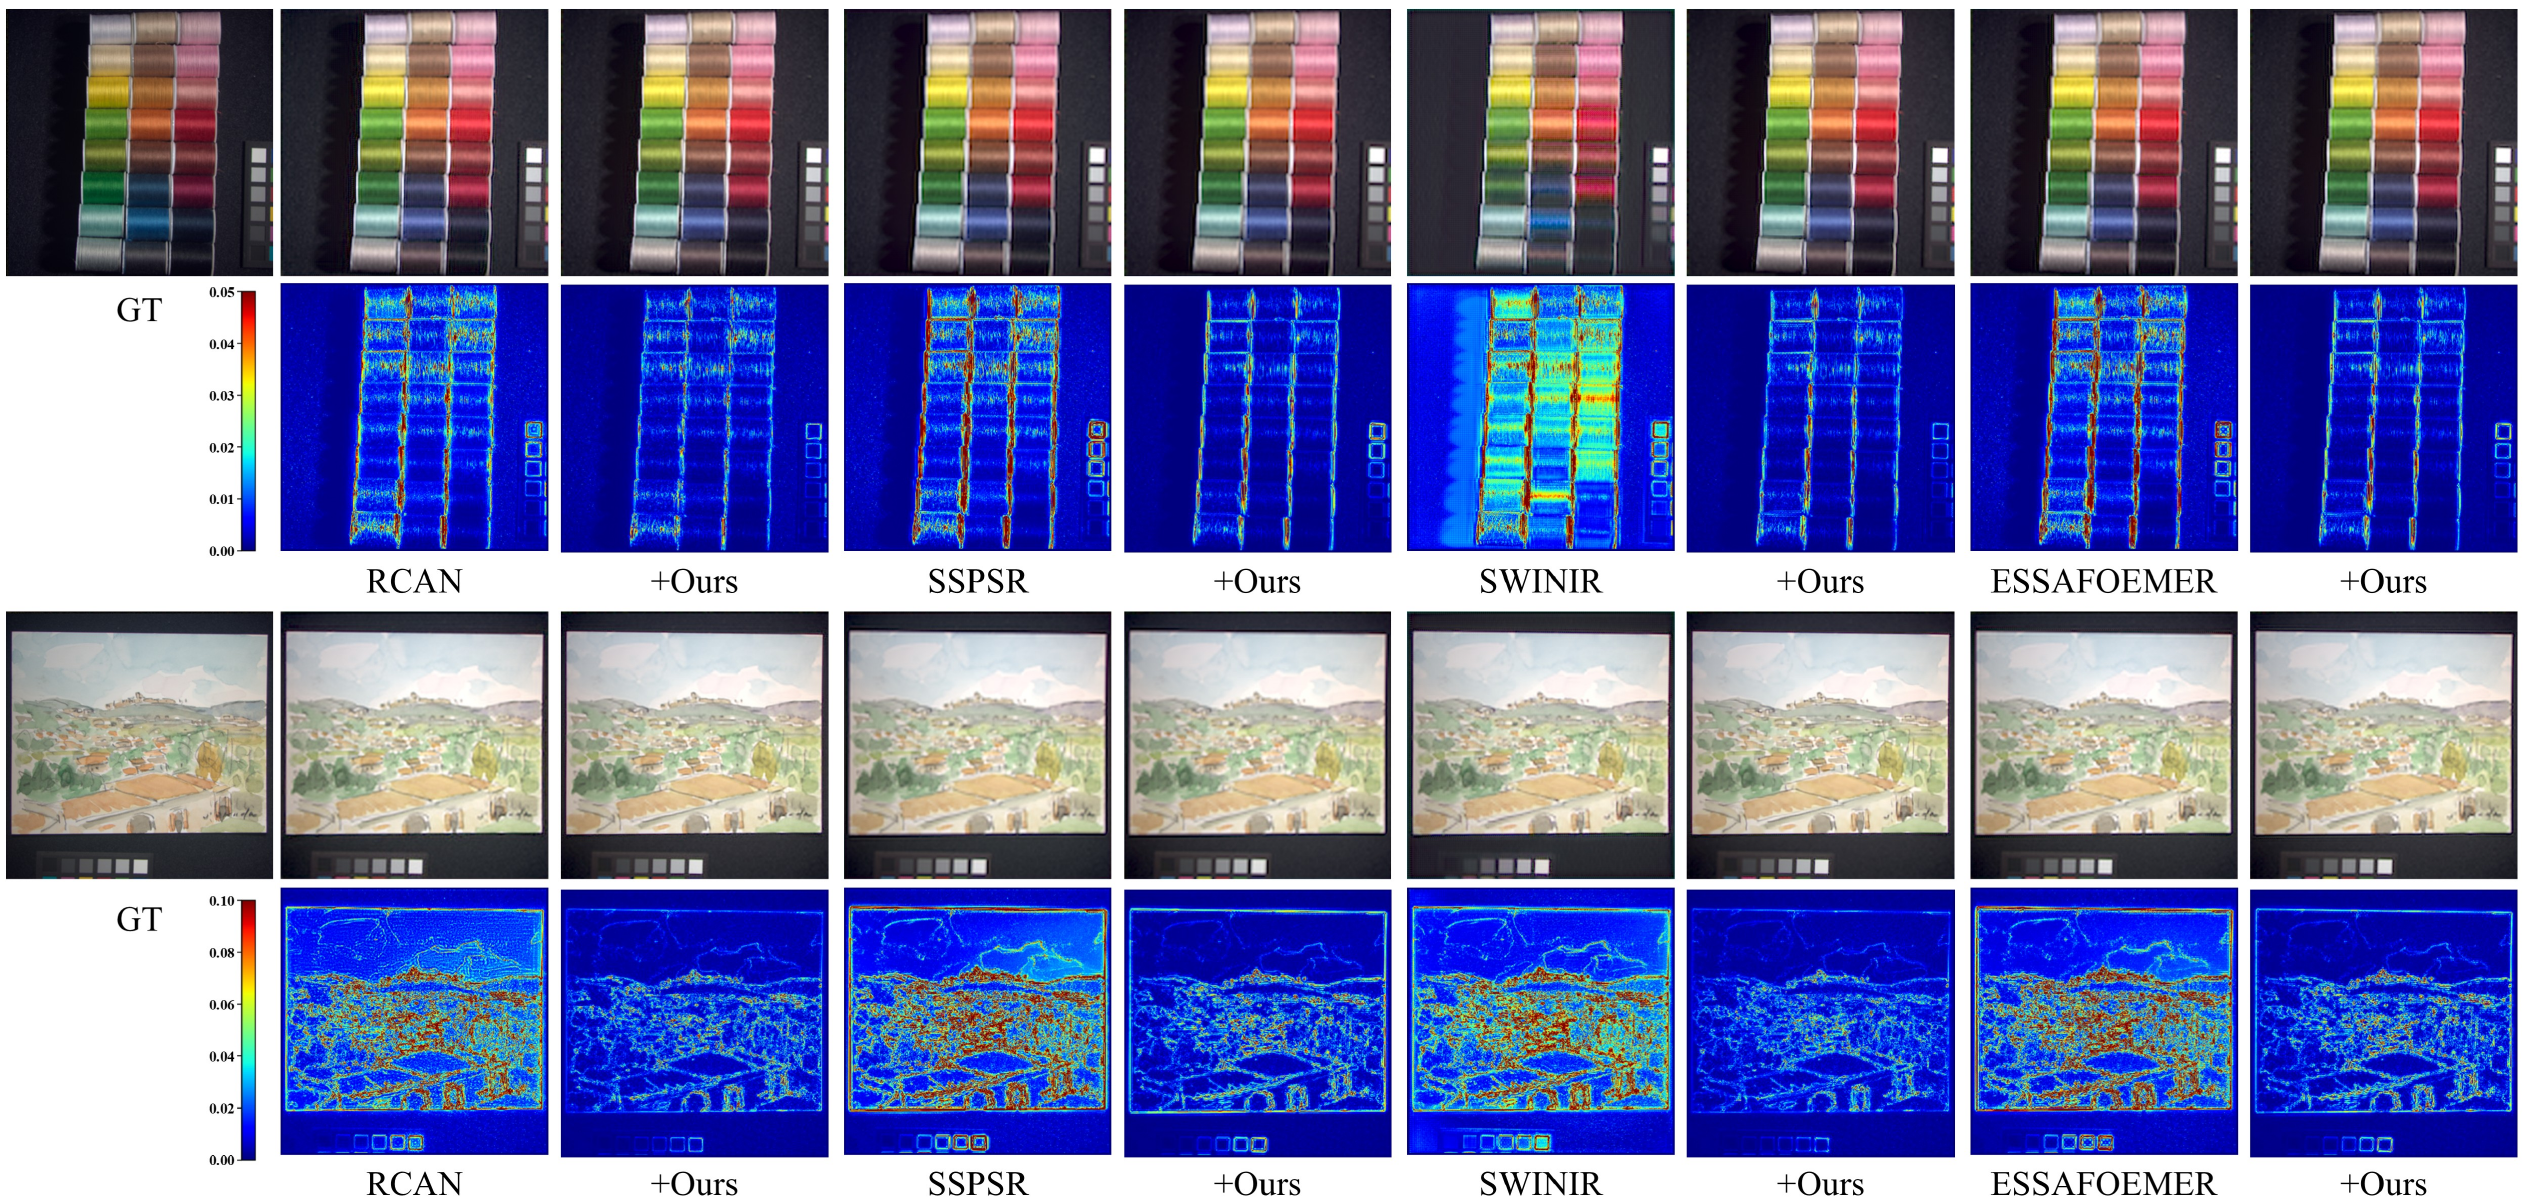}{fig:errmap_cave}

\ErrMapGalleryPage
{Representative error-map gallery on ICVL at $\times4$. The visualization protocol is identical to Fig.~\ref{fig:errmap_arad}.}
{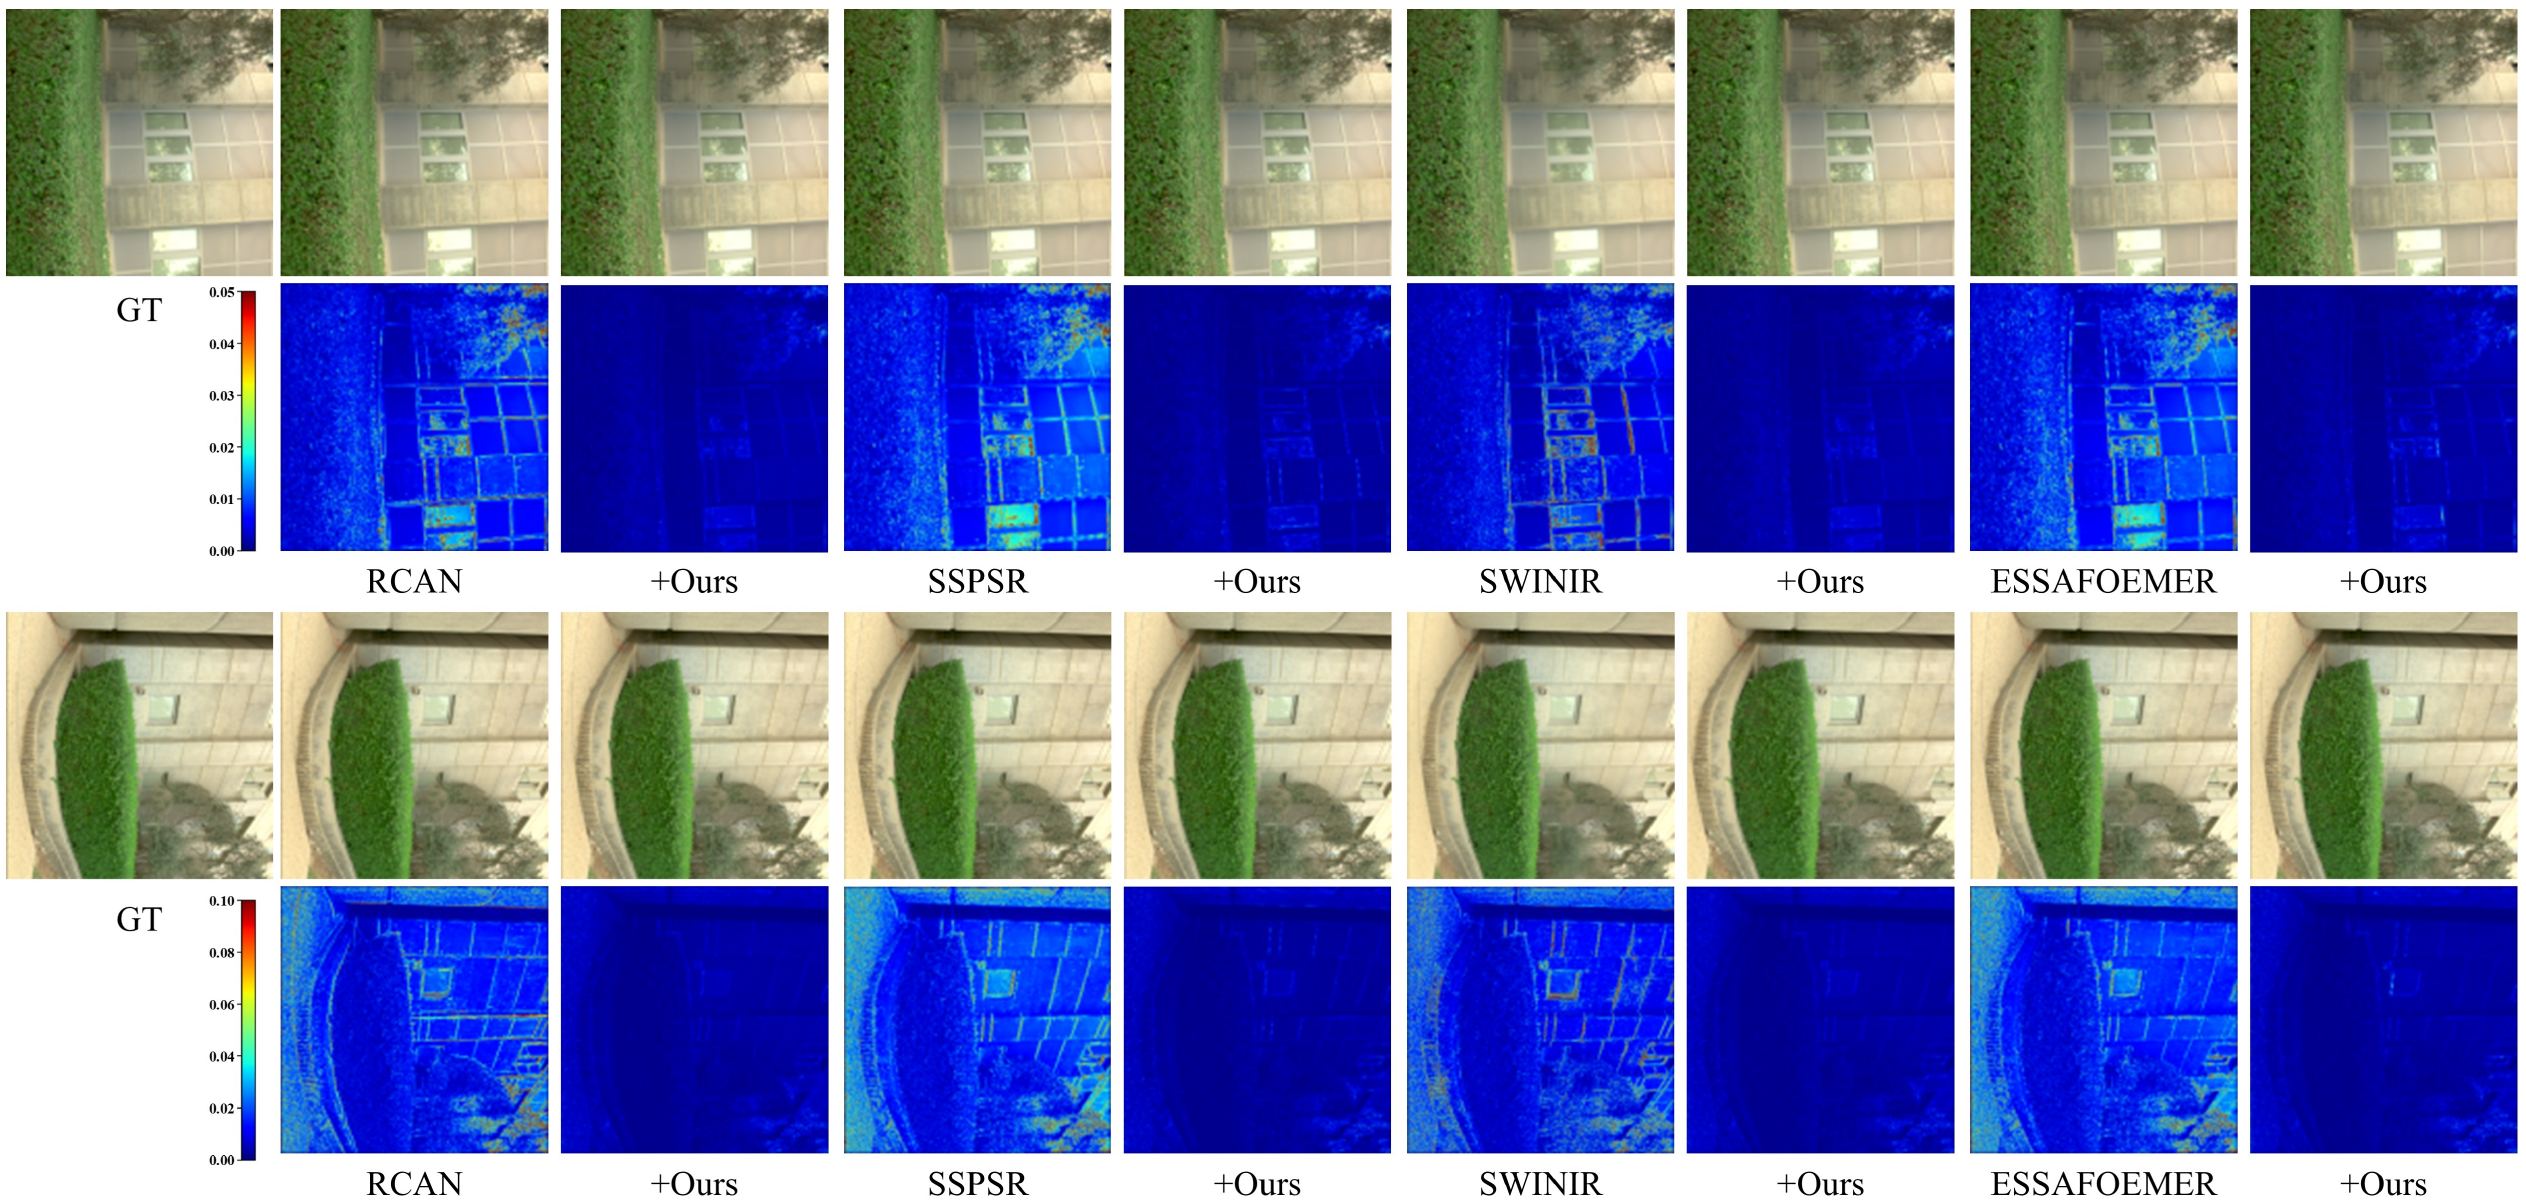}{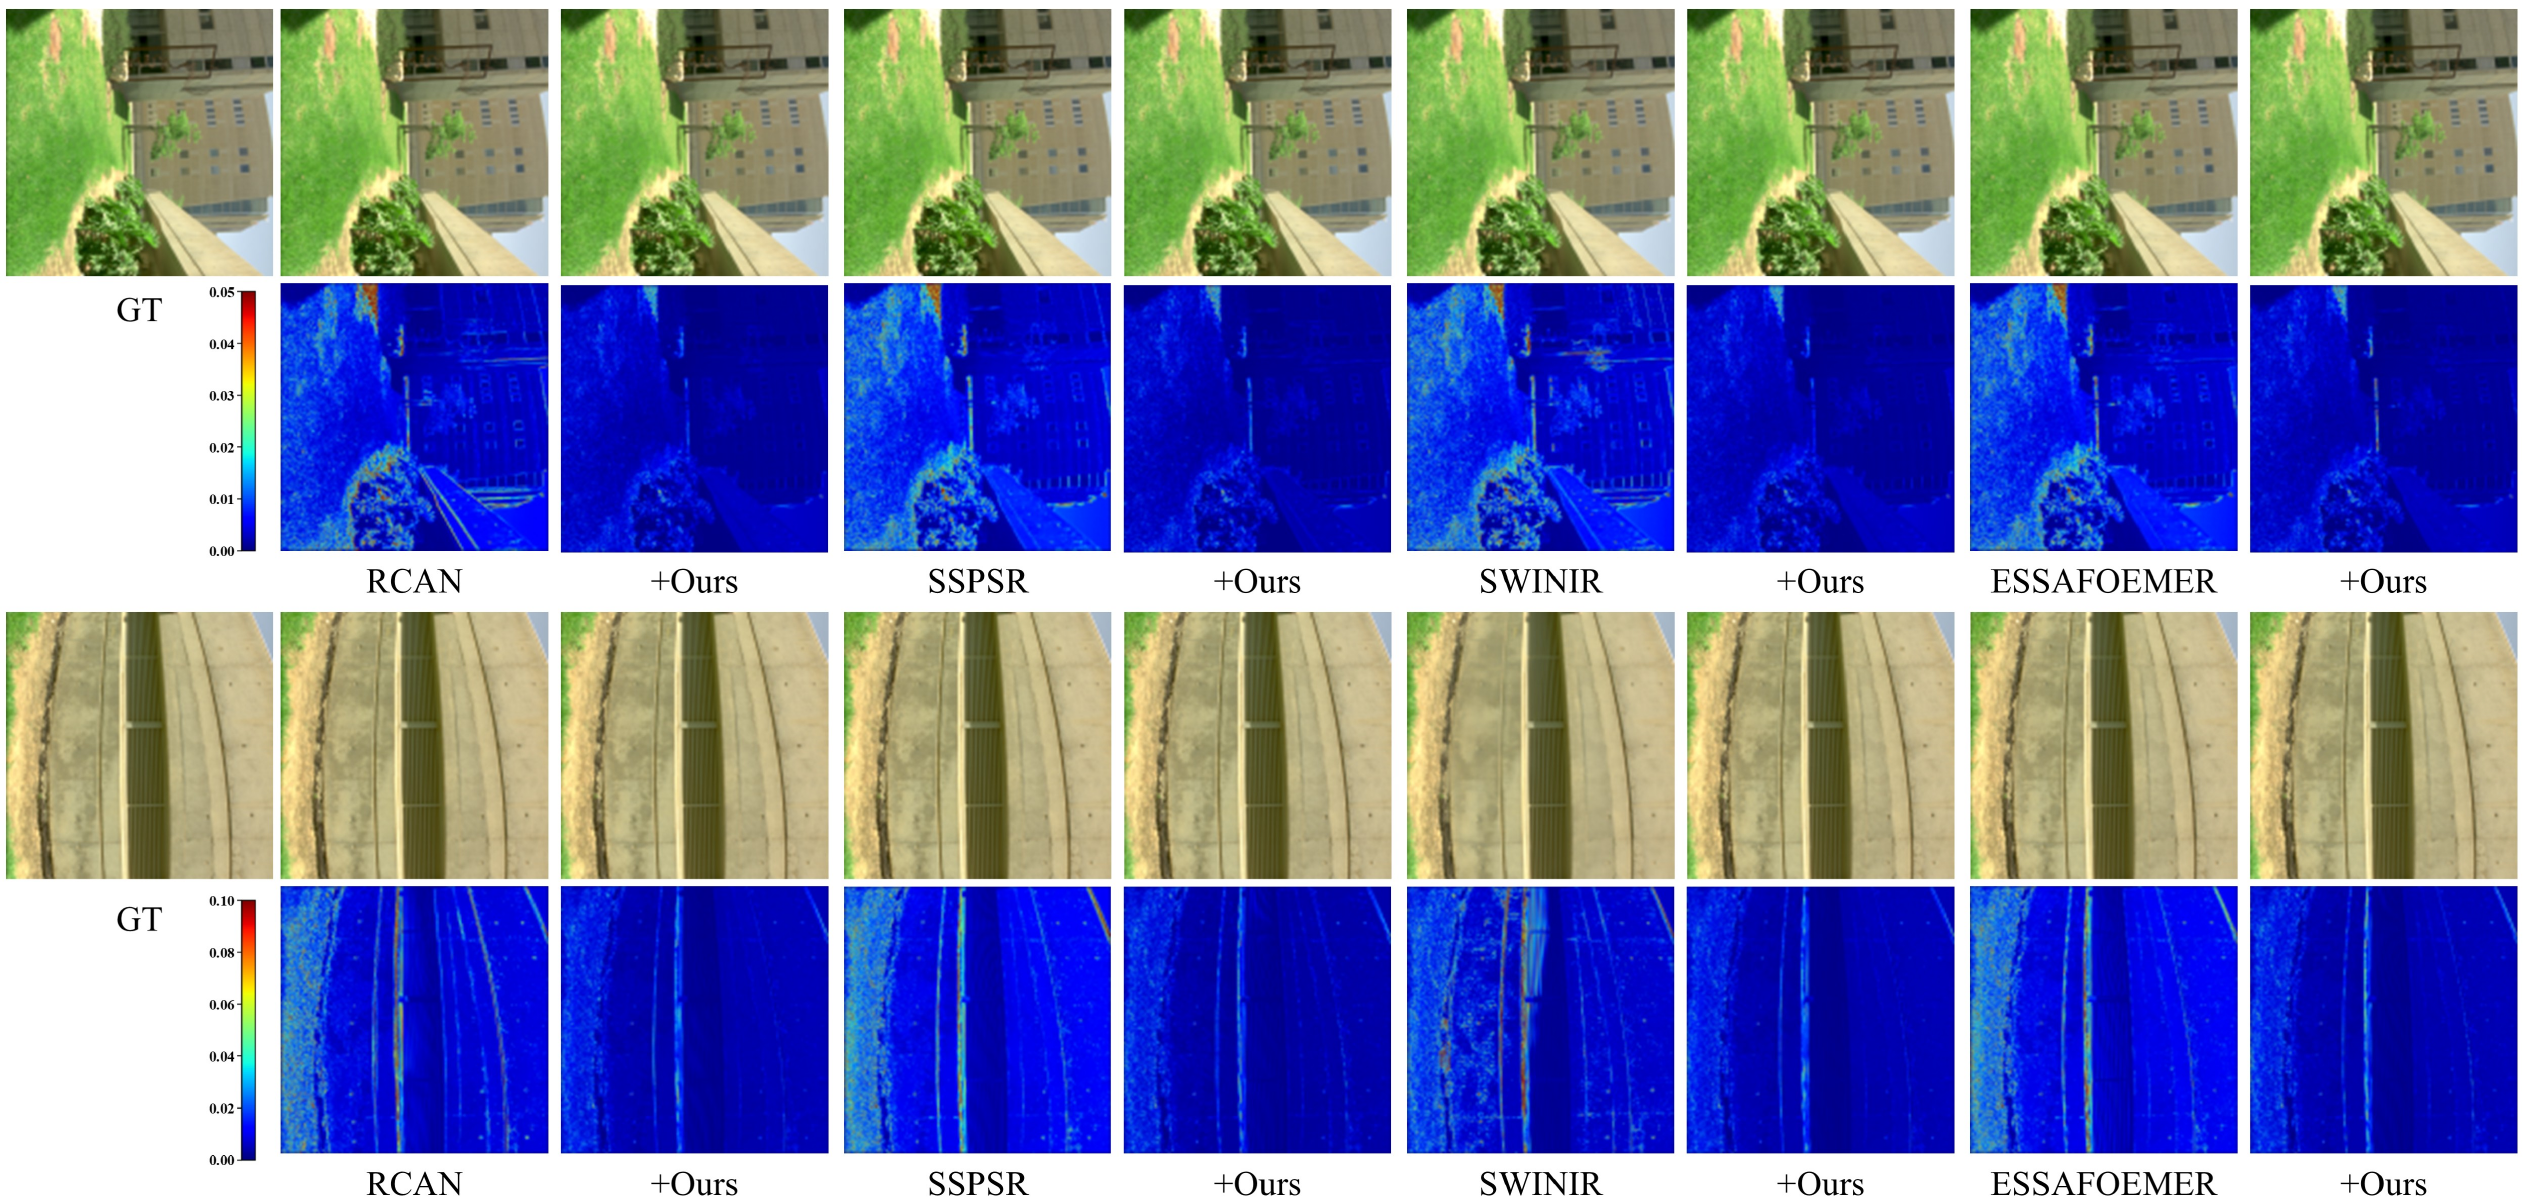}{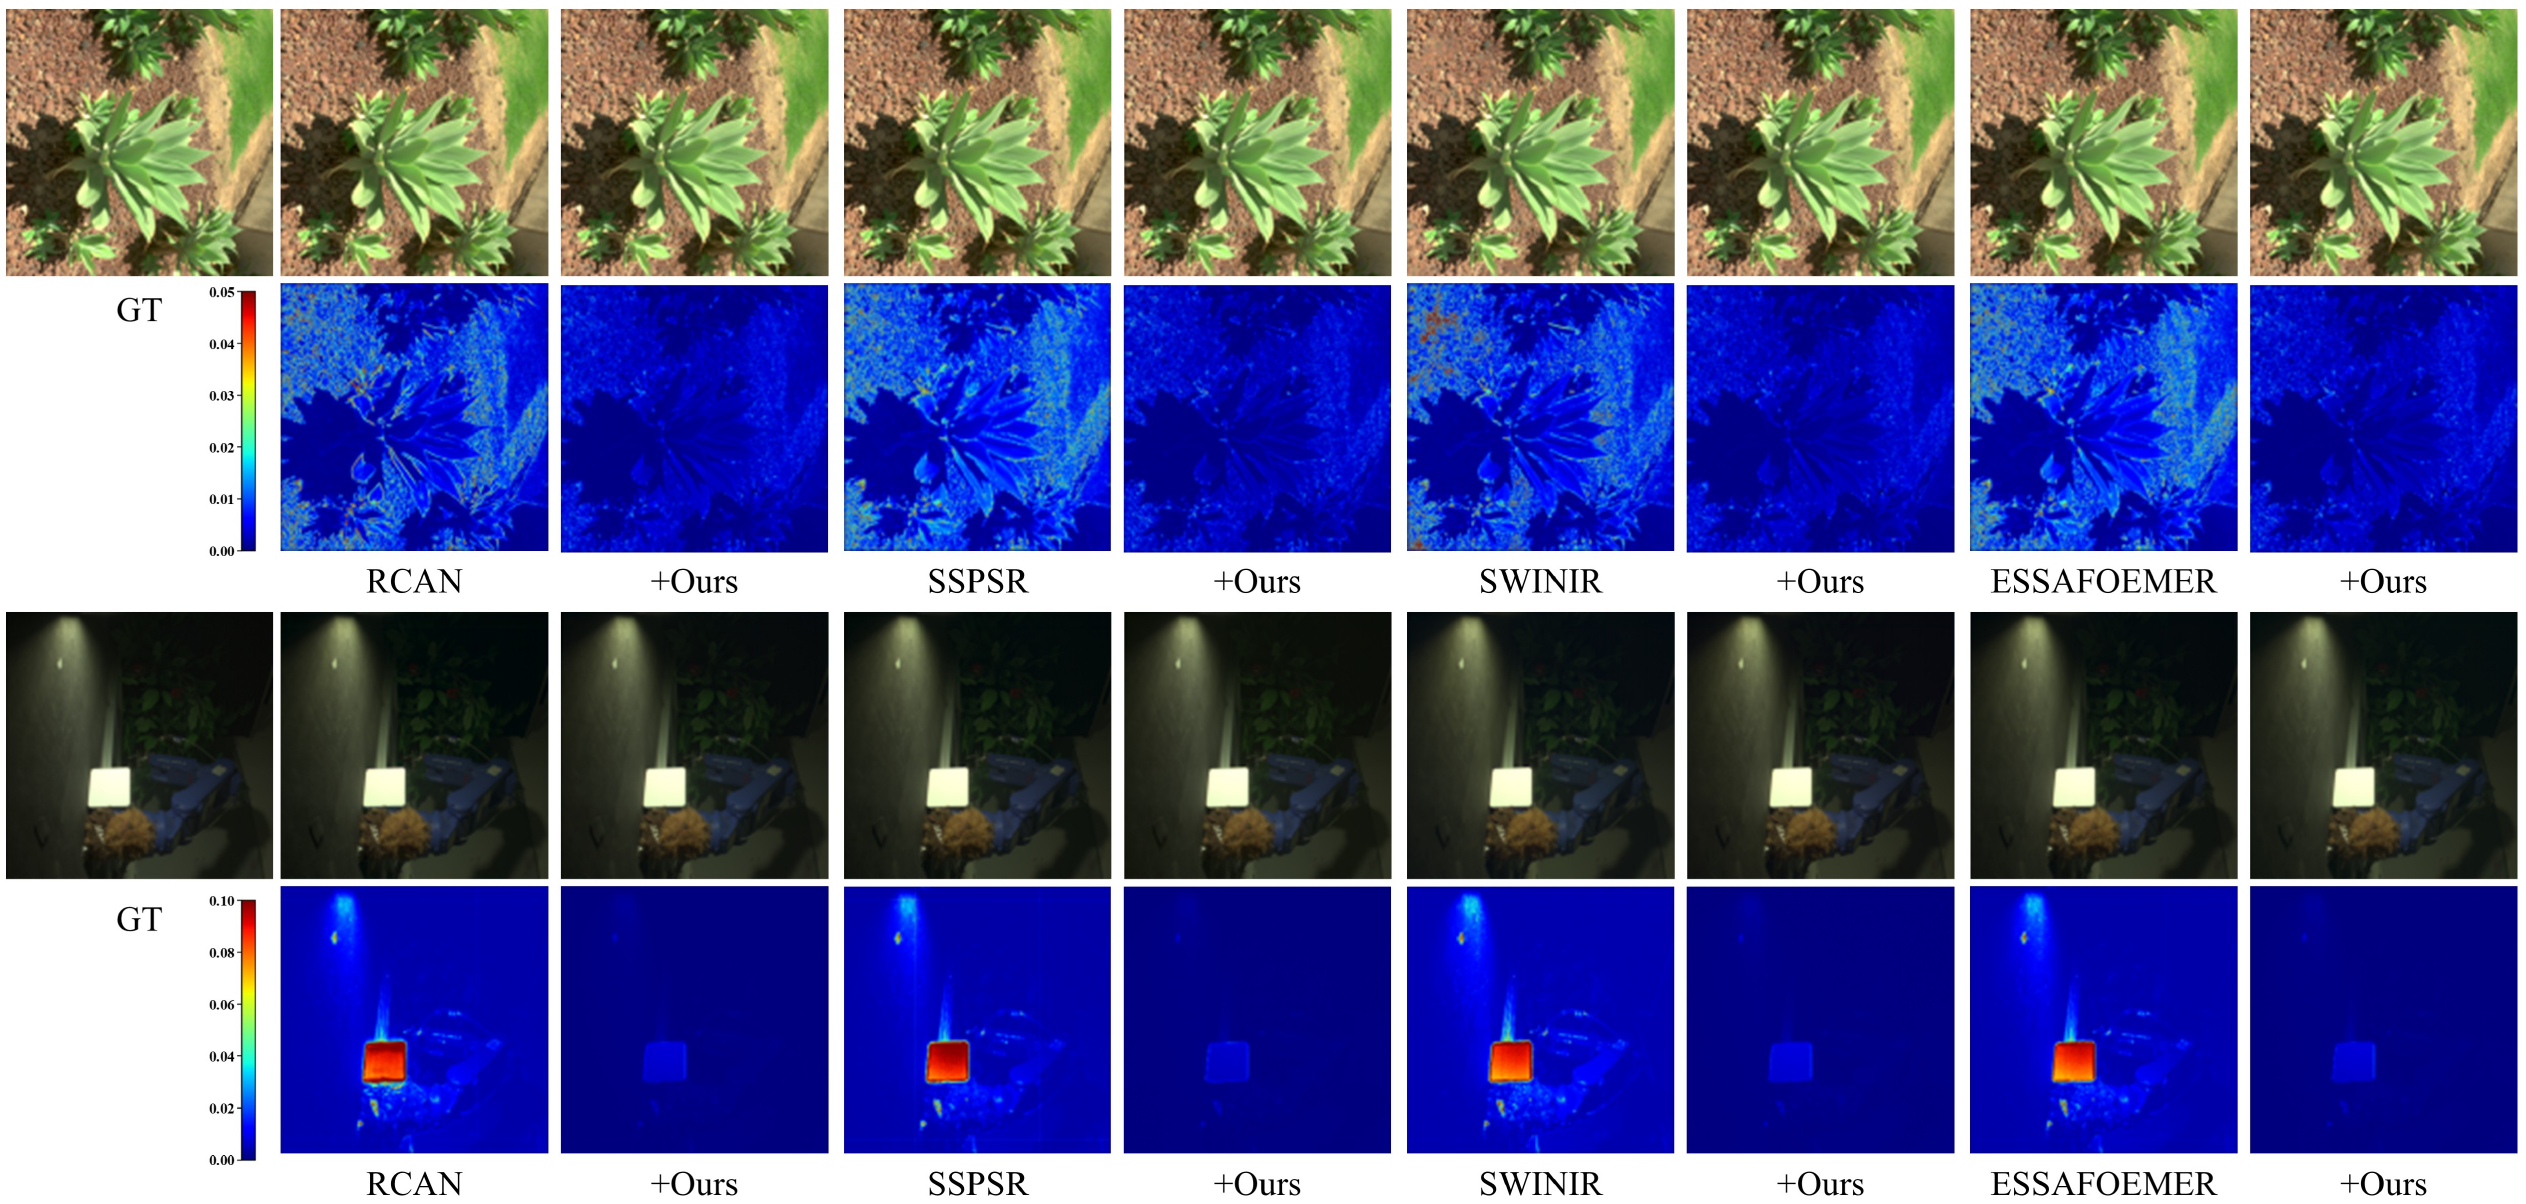}{fig:errmap_icvl}

\begin{table}[!t]
\centering

\scriptsize
\setlength{\tabcolsep}{4.6pt}        % <- 更宽的列间距（你可在 4.2~5.2 之间微调）
   % <- 更松的行距（1.05~1.15 都可）

\begin{adjustbox}{min width=\linewidth, max width=\linewidth}
\begin{tabular}{c c c|ccccccccc}
\toprule
Scale & Metric & Var. & K1 & K2 & B1 & B2 & N1 & N2 & N3 & J1 & J2 \\
\midrule

\multirow{9}{*}{$\times2$}
& \multirow{3}{*}{mPSNR} & Base  & 46.9930 & 45.2782 & 42.6891 & 39.8390 & 44.1997 & 42.8779 & 39.0326 & 41.2689 & 36.9781 \\
&                       & \ourscell{+Ours} & \ourscell{47.3542} & \ourscell{50.6912} & \ourscell{46.3376} & \ourscell{41.2105} & \ourscell{46.1393} & \ourscell{42.9718} & \ourscell{39.2598} & \ourscell{41.9803} & \ourscell{37.0884} \\
&                       & Gain  & \gainpos{+0.3612} & \gainpos{+5.4130} & \gainpos{+3.6485} & \gainpos{+1.3715} & \gainpos{+1.9396} & \gainpos{+0.0939} & \gainpos{+0.2272} & \gainpos{+0.7114} & \gainpos{+0.1103} \\
\cmidrule(lr){2-12}

& \multirow{3}{*}{mSSIM} & Base  & 0.9945 & 0.9917 & 0.9859 & 0.9742 & 0.9879 & 0.9806 & 0.9361 & 0.9754 & 0.9200 \\
&                        & \ourscell{+Ours} & \ourscell{0.9949} & \ourscell{0.9968} & \ourscell{0.9934} & \ourscell{0.9810} & \ourscell{0.9892} & \ourscell{0.9807} & \ourscell{0.9408} & \ourscell{0.9766} & \ourscell{0.9270} \\
&                        & Gain  & \gainpos{+0.0004} & \gainpos{+0.0051} & \gainpos{+0.0075} & \gainpos{+0.0068} & \gainpos{+0.0013} & \gainpos{+0.0001} & \gainpos{+0.0047} & \gainpos{+0.0012} & \gainpos{+0.0070} \\
\cmidrule(lr){2-12}

& \multirow{3}{*}{mSAM} & Base  & 0.6412 & 0.7029 & 0.8262 & 1.0349 & 2.2169 & 3.8313 & 7.6378 & 3.8589 & 7.6421 \\
&                       & \ourscell{+Ours} & \ourscell{0.5743} & \ourscell{0.5793} & \ourscell{0.6685} & \ourscell{0.9354} & \ourscell{2.0748} & \ourscell{3.7932} & \ourscell{6.3217} & \ourscell{3.7346} & \ourscell{7.2463} \\
&                       & Gain  & \gainpos{+0.0669} & \gainpos{+0.1236} & \gainpos{+0.1577} & \gainpos{+0.0995} & \gainpos{+0.1421} & \gainpos{+0.0381} & \gainpos{+1.3161} & \gainpos{+0.1243} & \gainpos{+0.3958} \\

\midrule

\multirow{9}{*}{$\times4$}
& \multirow{3}{*}{mPSNR} & Base  & 38.0659 & 37.3518 & 37.0133 & 36.4237 & 36.9821 & 36.6436 & 35.2832 & 36.3791 & 34.7529 \\
&                       & \ourscell{+Ours} & \ourscell{38.7683} & \ourscell{40.8013} & \ourscell{40.4649} & \ourscell{39.2507} & \ourscell{39.2291} & \ourscell{38.0369} & \ourscell{35.9106} & \ourscell{37.9000} & \ourscell{35.3443} \\
&                       & Gain  & \gainpos{+0.7024} & \gainpos{+3.4495} & \gainpos{+3.4516} & \gainpos{+2.8270} & \gainpos{+2.2470} & \gainpos{+1.3933} & \gainpos{+0.6274} & \gainpos{+1.5209} & \gainpos{+0.5914} \\
\cmidrule(lr){2-12}

& \multirow{3}{*}{mSSIM} & Base  & 0.9596 & 0.9531 & 0.9498 & 0.9437 & 0.9464 & 0.9395 & 0.9024 & 0.9367 & 0.8948 \\
&                        & \ourscell{+Ours} & \ourscell{0.9670} & \ourscell{0.9748} & \ourscell{0.9731} & \ourscell{0.9672} & \ourscell{0.9618} & \ourscell{0.9464} & \ourscell{0.9086} & \ourscell{0.9452} & \ourscell{0.8970} \\
&                        & Gain  & \gainpos{+0.0074} & \gainpos{+0.0217} & \gainpos{+0.0233} & \gainpos{+0.0235} & \gainpos{+0.0154} & \gainpos{+0.0069} & \gainpos{+0.0062} & \gainpos{+0.0085} & \gainpos{+0.0022} \\
\cmidrule(lr){2-12}

& \multirow{3}{*}{mSAM} & Base  & 1.3722 & 1.4583 & 1.4760 & 1.5187 & 2.5611 & 3.8740 & 7.0666 & 3.8760 & 7.0590 \\
&                       & \ourscell{+Ours} & \ourscell{1.3204} & \ourscell{1.2944} & \ourscell{1.2709} & \ourscell{1.2949} & \ourscell{2.2280} & \ourscell{3.2619} & \ourscell{6.8138} & \ourscell{3.2247} & \ourscell{6.8102} \\
&                       & Gain  & \gainpos{+0.0518} & \gainpos{+0.1639} & \gainpos{+0.2051} & \gainpos{+0.2238} & \gainpos{+0.3331} & \gainpos{+0.6121} & \gainpos{+0.2528} & \gainpos{+0.6513} & \gainpos{+0.2488} \\

\midrule

\multirow{9}{*}{$\times8$}
& \multirow{3}{*}{mPSNR} & Base  & 32.6296 & 32.3557 & 32.3143 & 32.2368 & 32.0617 & 31.8439 & 31.1646 & 31.7823 & 31.0966 \\
&                       & \ourscell{+Ours} & \ourscell{33.3445} & \ourscell{34.8300} & \ourscell{34.8294} & \ourscell{34.7736} & \ourscell{34.1853} & \ourscell{33.6229} & \ourscell{31.9019} & \ourscell{33.6025} & \ourscell{31.9108} \\
&                       & Gain  & \gainpos{+0.7149} & \gainpos{+2.4743} & \gainpos{+2.5151} & \gainpos{+2.5368} & \gainpos{+2.1236} & \gainpos{+1.7790} & \gainpos{+0.7373} & \gainpos{+1.8202} & \gainpos{+0.8142} \\
\cmidrule(lr){2-12}

& \multirow{3}{*}{mSSIM} & Base  & 0.8769 & 0.8698 & 0.8689 & 0.8672 & 0.8608 & 0.8526 & 0.8230 & 0.8518 & 0.8211 \\
&                        & \ourscell{+Ours} & \ourscell{0.8968} & \ourscell{0.9102} & \ourscell{0.9098} & \ourscell{0.9087} & \ourscell{0.8953} & \ourscell{0.8796} & \ourscell{0.8289} & \ourscell{0.8790} & \ourscell{0.8265} \\
&                        & Gain  & \gainpos{+0.0199} & \gainpos{+0.0404} & \gainpos{+0.0409} & \gainpos{+0.0415} & \gainpos{+0.0345} & \gainpos{+0.0270} & \gainpos{+0.0059} & \gainpos{+0.0272} & \gainpos{+0.0054} \\
\cmidrule(lr){2-12}

& \multirow{3}{*}{mSAM} & Base  & 2.3049 & 2.4180 & 2.4190 & 2.4220 & 3.0980 & 4.0295 & 6.5479 & 4.0262 & 6.5525 \\
&                       & \ourscell{+Ours} & \ourscell{2.2712} & \ourscell{2.1173} & \ourscell{2.1052} & \ourscell{2.0901} & \ourscell{2.8654} & \ourscell{3.5249} & \ourscell{6.3644} & \ourscell{3.5022} & \ourscell{5.9158} \\
&                       & Gain  & \gainpos{+0.0337} & \gainpos{+0.3007} & \gainpos{+0.3138} & \gainpos{+0.3319} & \gainpos{+0.2326} & \gainpos{+0.5046} & \gainpos{+0.1835} & \gainpos{+0.5240} & \gainpos{+0.6367} \\

\bottomrule
\end{tabular}
\end{adjustbox}
\caption{Robustness to mild test-time degradation mismatch on ARAD-1K.
We consider nine test-time settings grouped as kernel mismatch (K1: area downsampling; K2: an alternative bicubic implementation),
blur mismatch (B1/B2: HR-space Gaussian blur with $\sigma\in\{0.6,1.0\}$ using $5\times5$ and $7\times7$ kernels before bicubic downsampling),
noise mismatch (N1/N2/N3: i.i.d.\ Gaussian noise added in LR after downsampling with $\sigma=n/255$ for $n\in\{1,2,5\}$),
and combined blur+noise mismatch (J1/J2: $(\sigma,n)\in\{(0.6,2),(1.0,5)\}$).
Gain is computed as (+Ours $-$ Base) for mPSNR/mSSIM and (Base $-$ +Ours) for mSAM.}
\label{tab:app_deg_results_arad_compact}
\end{table}

\begin{table}[htbp]
\centering
\scriptsize
% 这两个参数决定“宽/高的观感”，推荐从这里微调
\setlength{\tabcolsep}{2.8pt}   % 建议 2.6--3.2
 % 建议 1.00--1.08

\begin{adjustbox}{min width=\linewidth, max width=\linewidth}
\begin{tabular}{l|cccc|cccc|cccc}
\toprule
\multirow{2}{*}{Method} &
\multicolumn{4}{c|}{$\times2$} &
\multicolumn{4}{c|}{$\times4$} &
\multicolumn{4}{c}{$\times8$} \\
\cmidrule(lr){2-5}\cmidrule(lr){6-9}\cmidrule(lr){10-13}
& mPSNR$\uparrow$ & mSAM$\downarrow$ & mSSIM$\uparrow$ & CC$\uparrow$
& mPSNR$\uparrow$ & mSAM$\downarrow$ & mSSIM$\uparrow$ & CC$\uparrow$
& mPSNR$\uparrow$ & mSAM$\downarrow$ & mSSIM$\uparrow$ & CC$\uparrow$ \\
\midrule
Base (SwinIR)
& 50.4662 & 0.7727 & 0.9972 & 0.9990
& 39.5717 & 1.3950 & 0.9709 & 0.9902
& 32.5185 & 2.4680 & 0.8869 & 0.9551 \\
Base + SG
& 46.1893 & 1.9059 & 0.9959 & 0.9975
& 38.7834 & 2.4512 & 0.9698 & 0.9889
& 32.3362 & 3.2638 & 0.8859 & 0.9541 \\
Base + PCA
& 50.7837 & 0.6188 & 0.9972 & 0.9990
& 39.5729 & 1.4028 & 0.9709 & 0.9902
& 32.5198 & 2.4601 & 0.8869 & 0.9552 \\
Base + IBP
& 51.0962 & 0.5211 & 0.9973 & 0.9992
& 39.5782 & 1.3693 & 0.9709 & 0.9902
& 32.5041 & 2.4365 & 0.8865 & 0.9548 \\
Base + MCR
& \gainpos{51.2531} & \gainpos{0.5182} & \gainpos{0.9973} & \gainpos{0.9992}
& \gainpos{40.2550} & \gainpos{1.3173} & \gainpos{0.9752} & \gainpos{0.9912}
& \gainpos{33.9241} & \gainpos{2.2159} & \gainpos{0.8947} & \gainpos{0.9675} \\
\rowcolor{oursgray}
Base + Ours
& 51.6551 & 0.4842 & 0.9975 & 0.9993
& 40.9720 & 1.2819 & 0.9752 & 0.9924
& 34.8318 & 2.1164 & 0.9103 & 0.9720 \\
\bottomrule
\end{tabular}
\end{adjustbox}
\caption{Comparison to simple spectral rectifiers on ARAD using SwinIR at $\times2$, $\times4$, and $\times8$.
SG/PCA/IBP are applied post hoc to the fixed SwinIR output.
MCR is our proposed rectification module (a component of~\name) evaluated as a standalone post hoc rectifier, while \name is trained end-to-end.}
\label{tab:app_simple_rectifiers}
\end{table}

% ---------- ARAD: 3 PDFs in one page ----------
\begin{figure}[p]
\centering
\includegraphics[width=\linewidth,height=0.285\textheight,keepaspectratio]{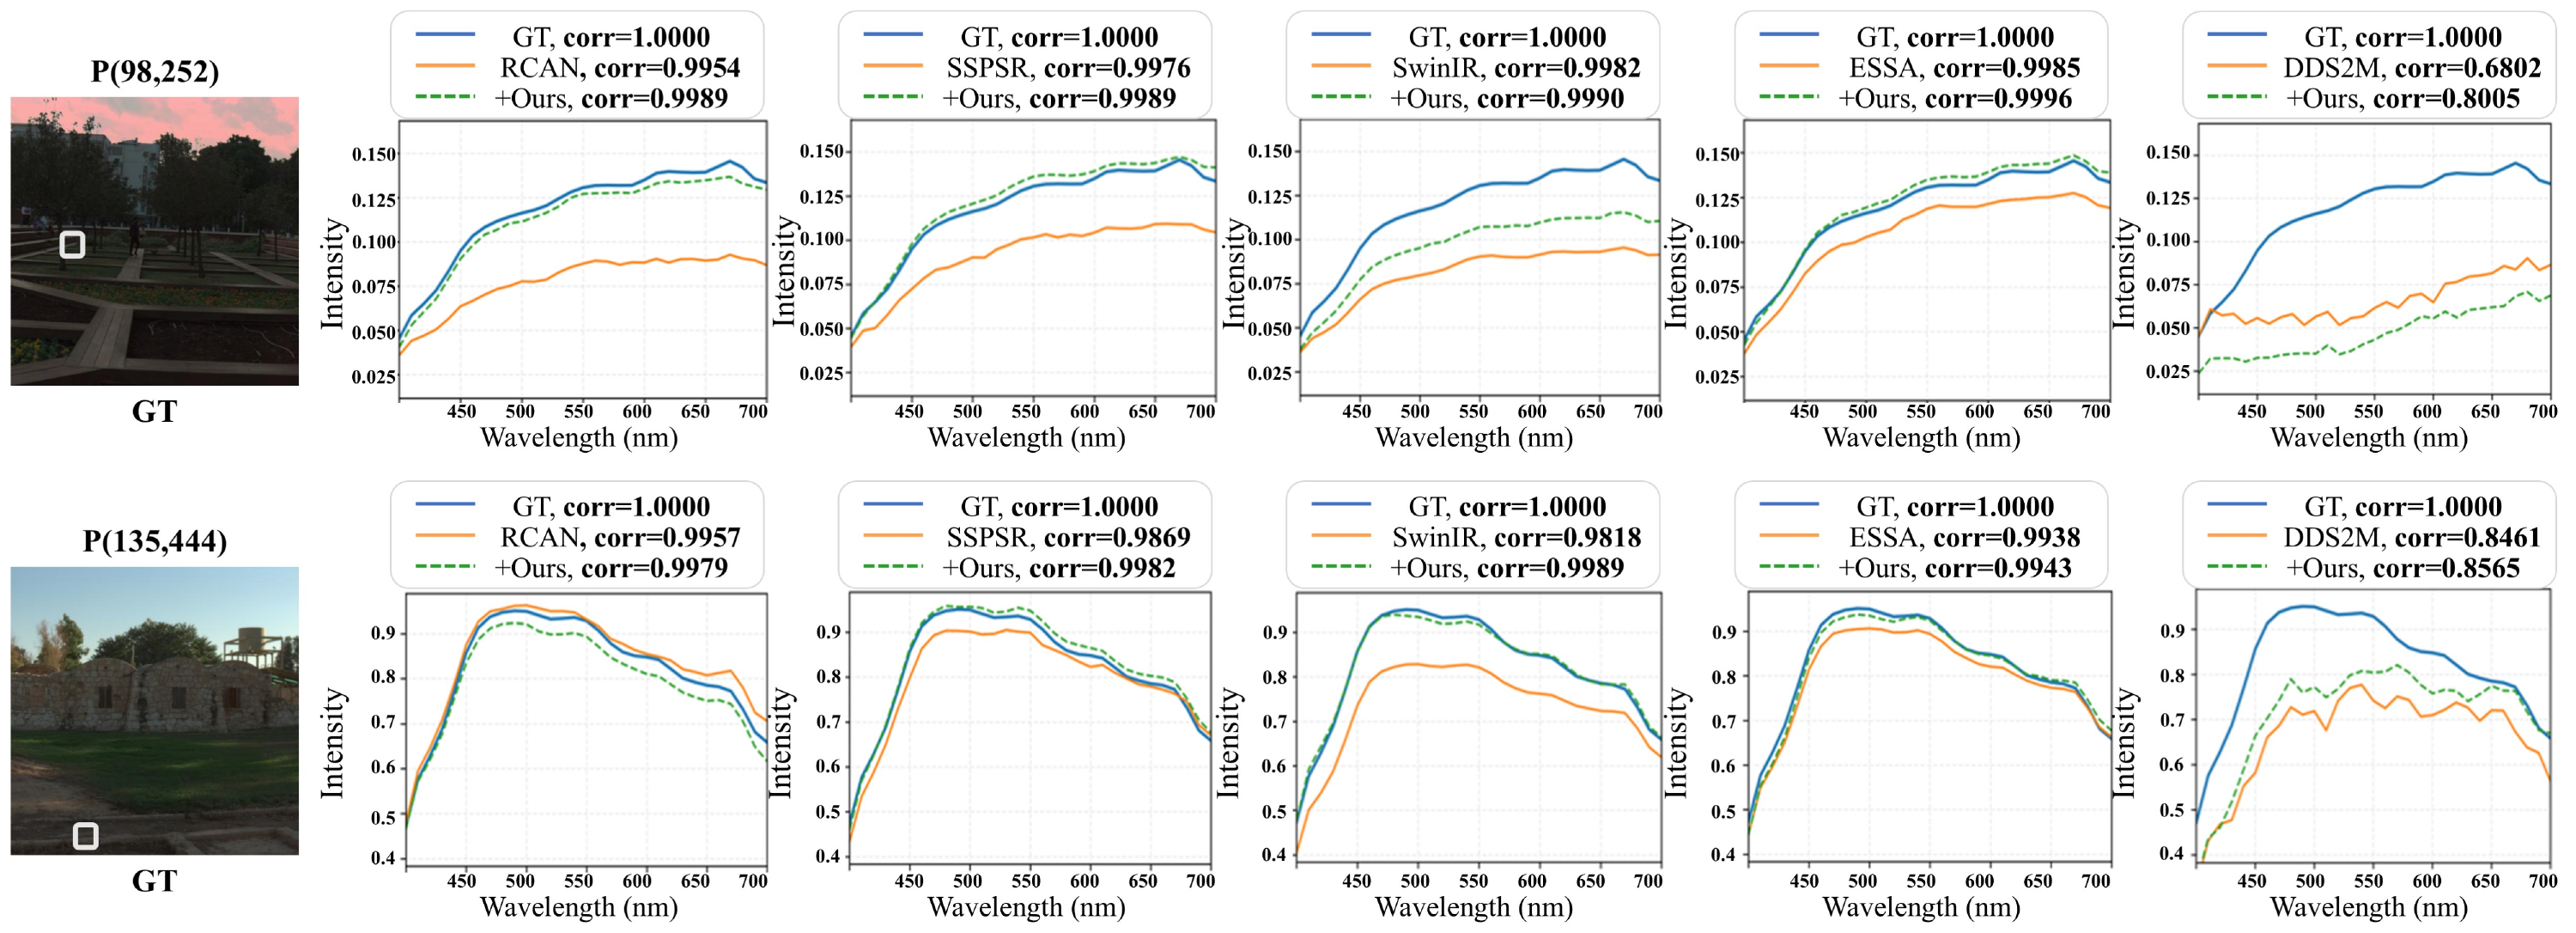}\vspace{2pt}
\includegraphics[width=\linewidth,height=0.285\textheight,keepaspectratio]{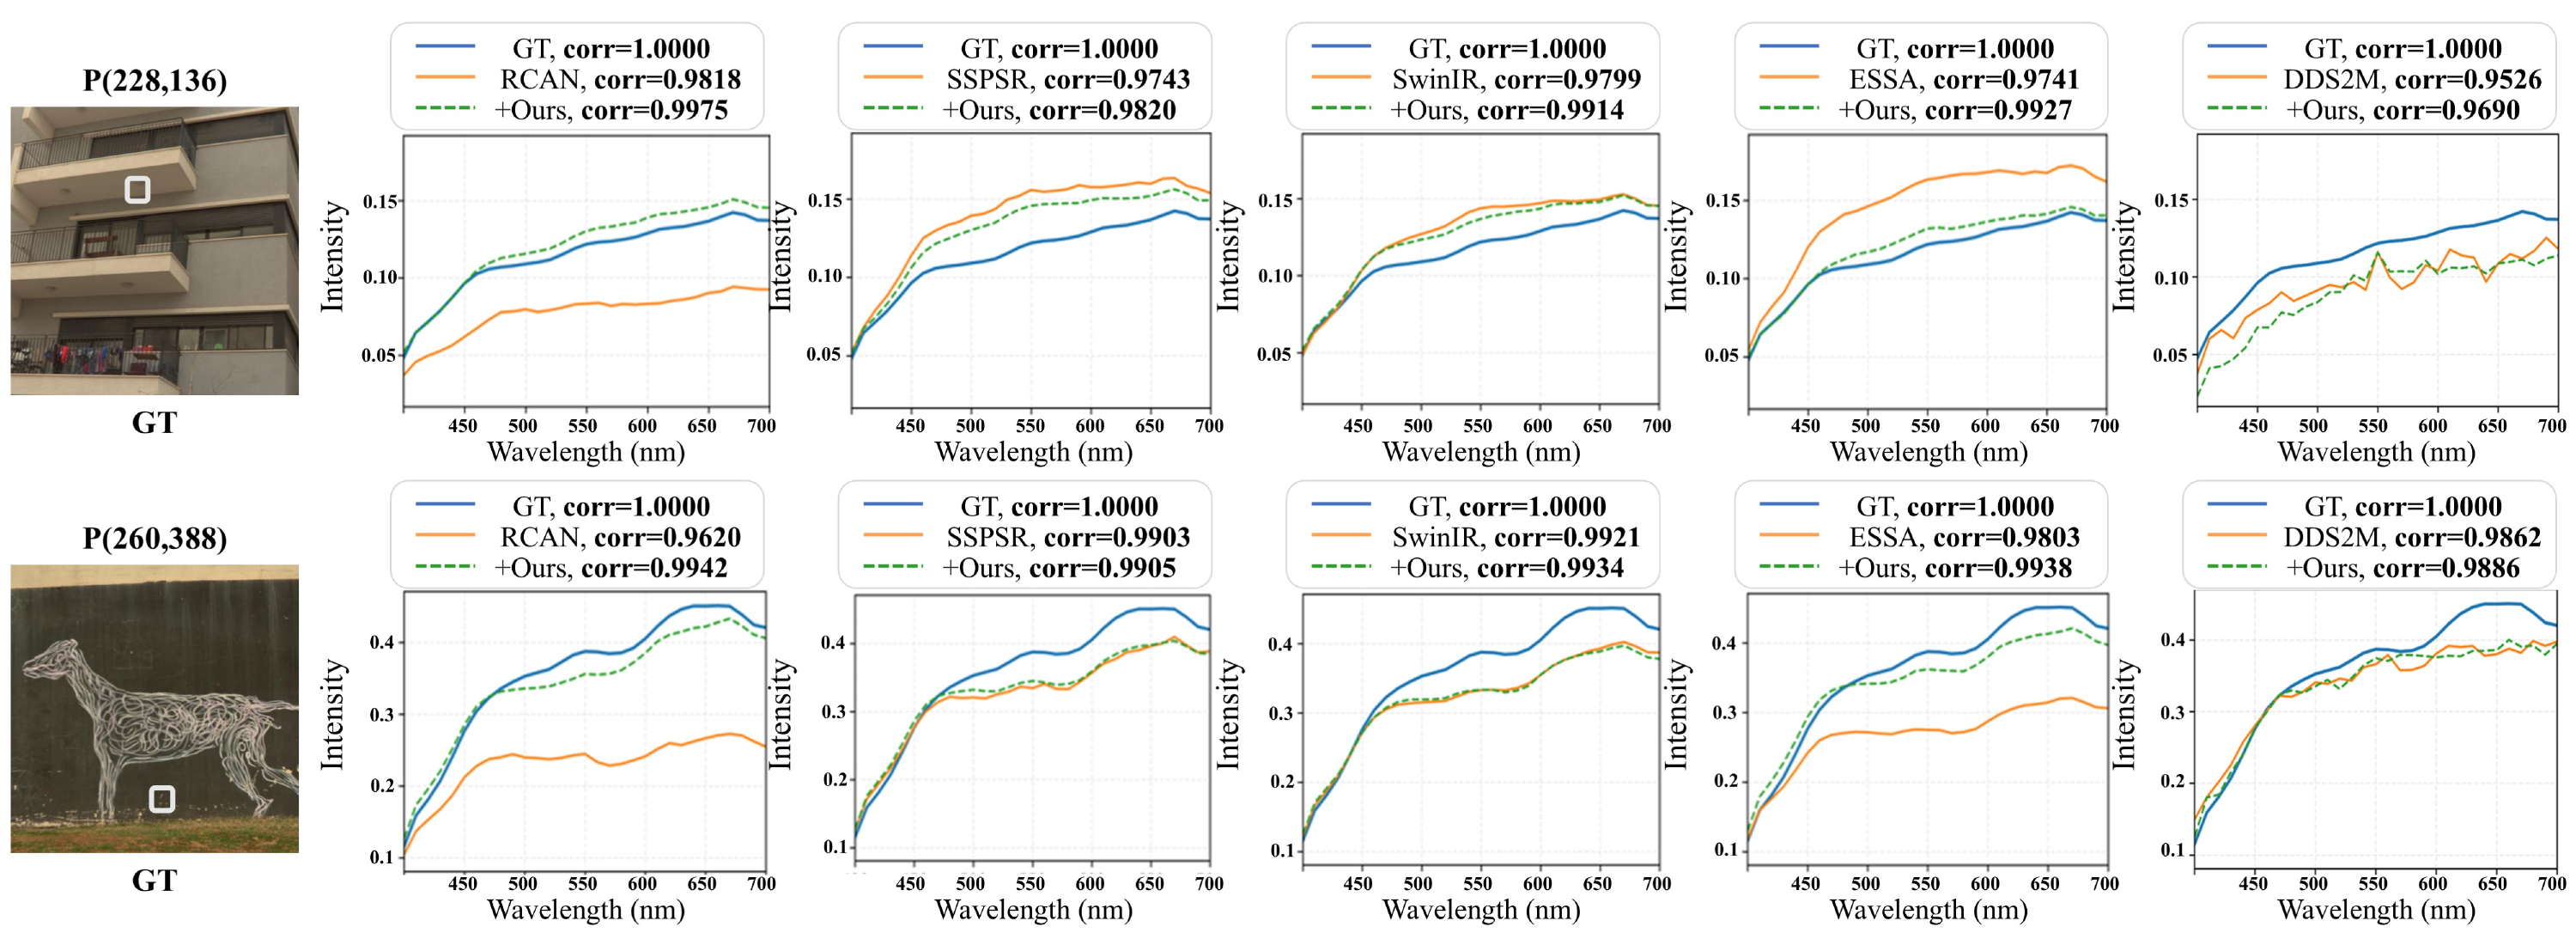}\vspace{2pt}
\includegraphics[width=\linewidth,height=0.285\textheight,keepaspectratio]{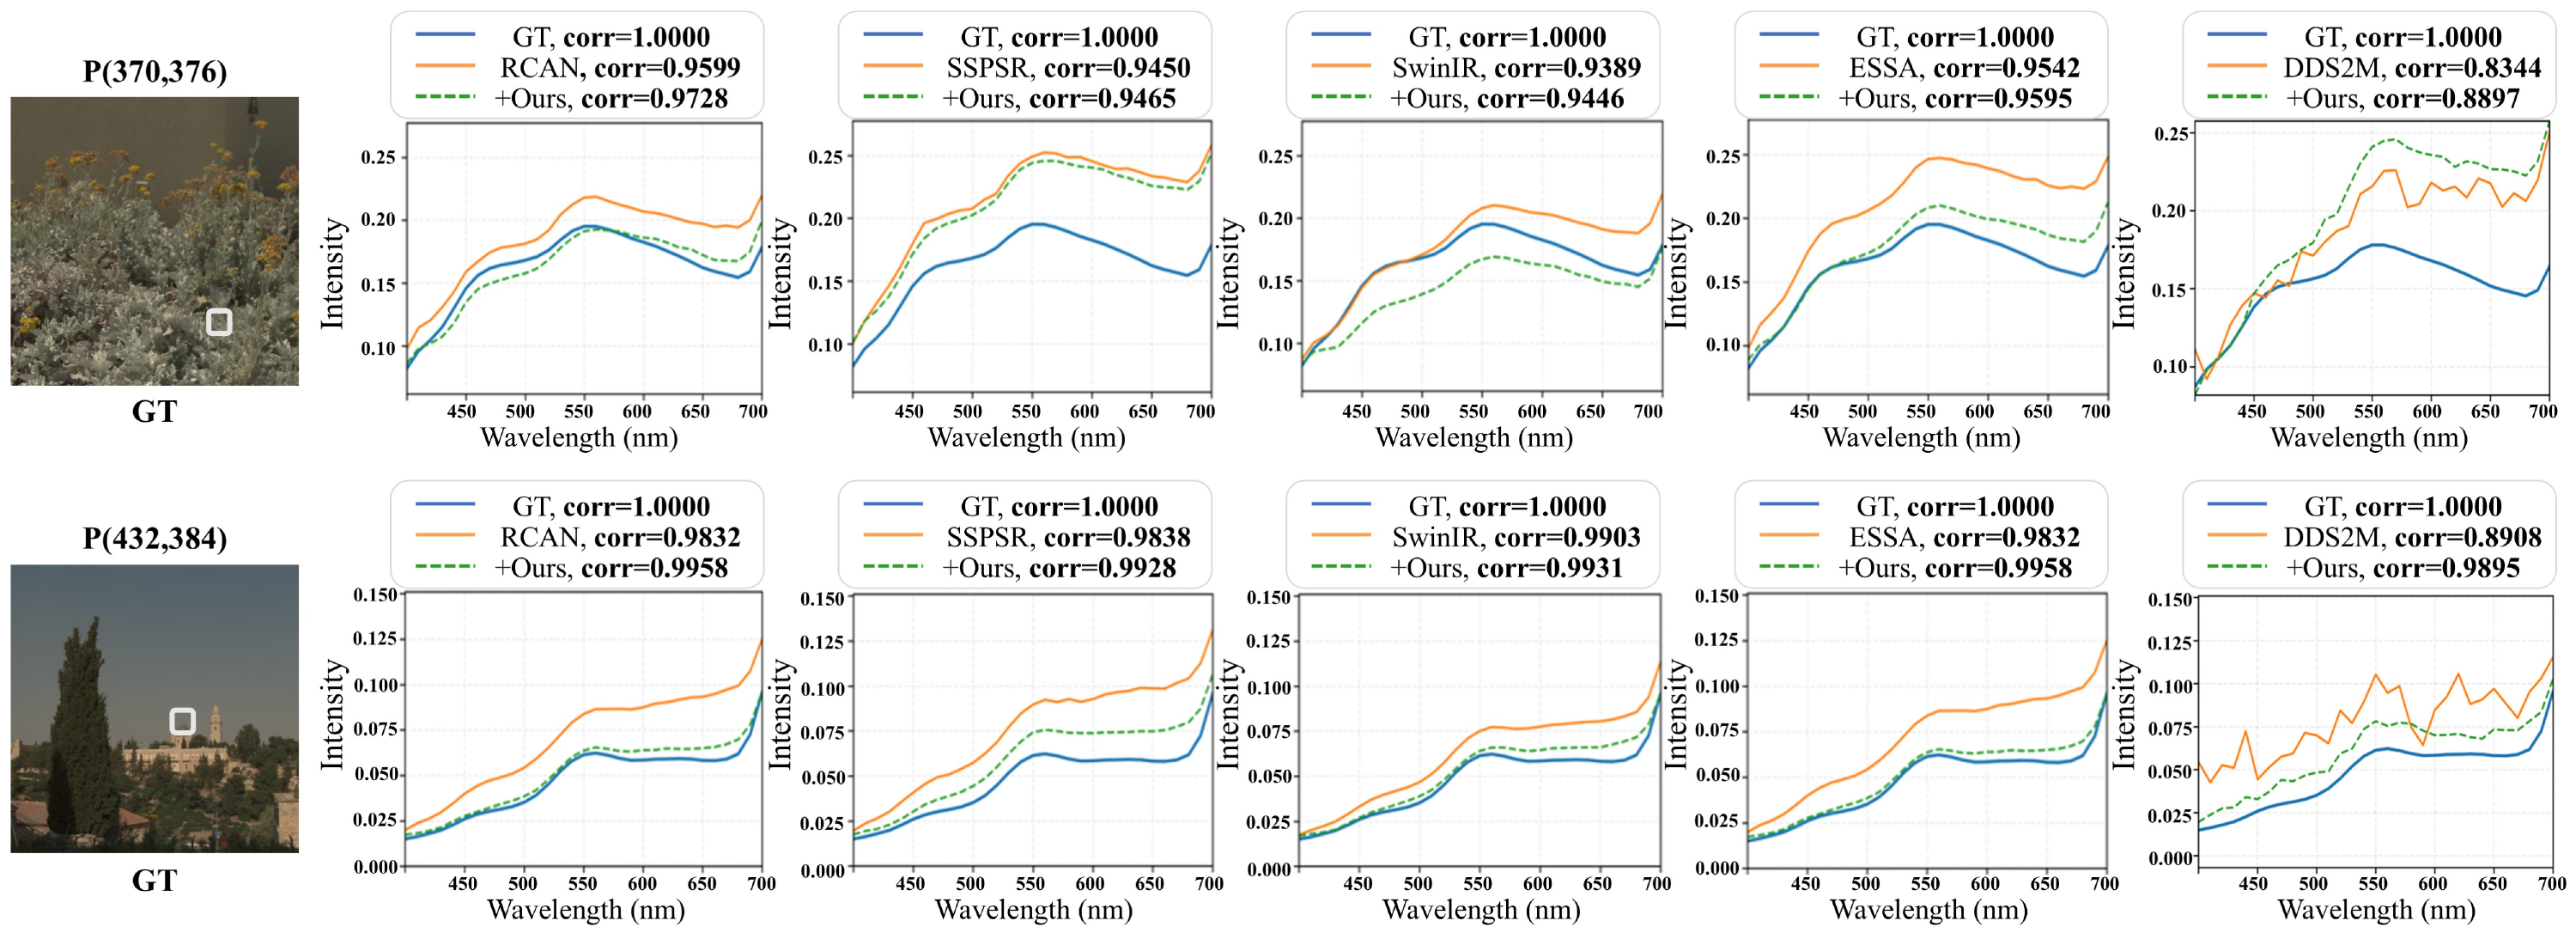}

\caption{Additional spectral curve gallery on ARAD-1K at $\times4$. Curves include CNN-, Transformer-, and diffusion-based backbones, including DDS2M.}
\label{fig:sp_arad_gallery}
\end{figure}

\FloatBarrier

% ---------- CAVE: 3 PDFs in one page ----------
\begin{figure}[!p]
\centering
\includegraphics[width=\linewidth,height=0.285\textheight,keepaspectratio]{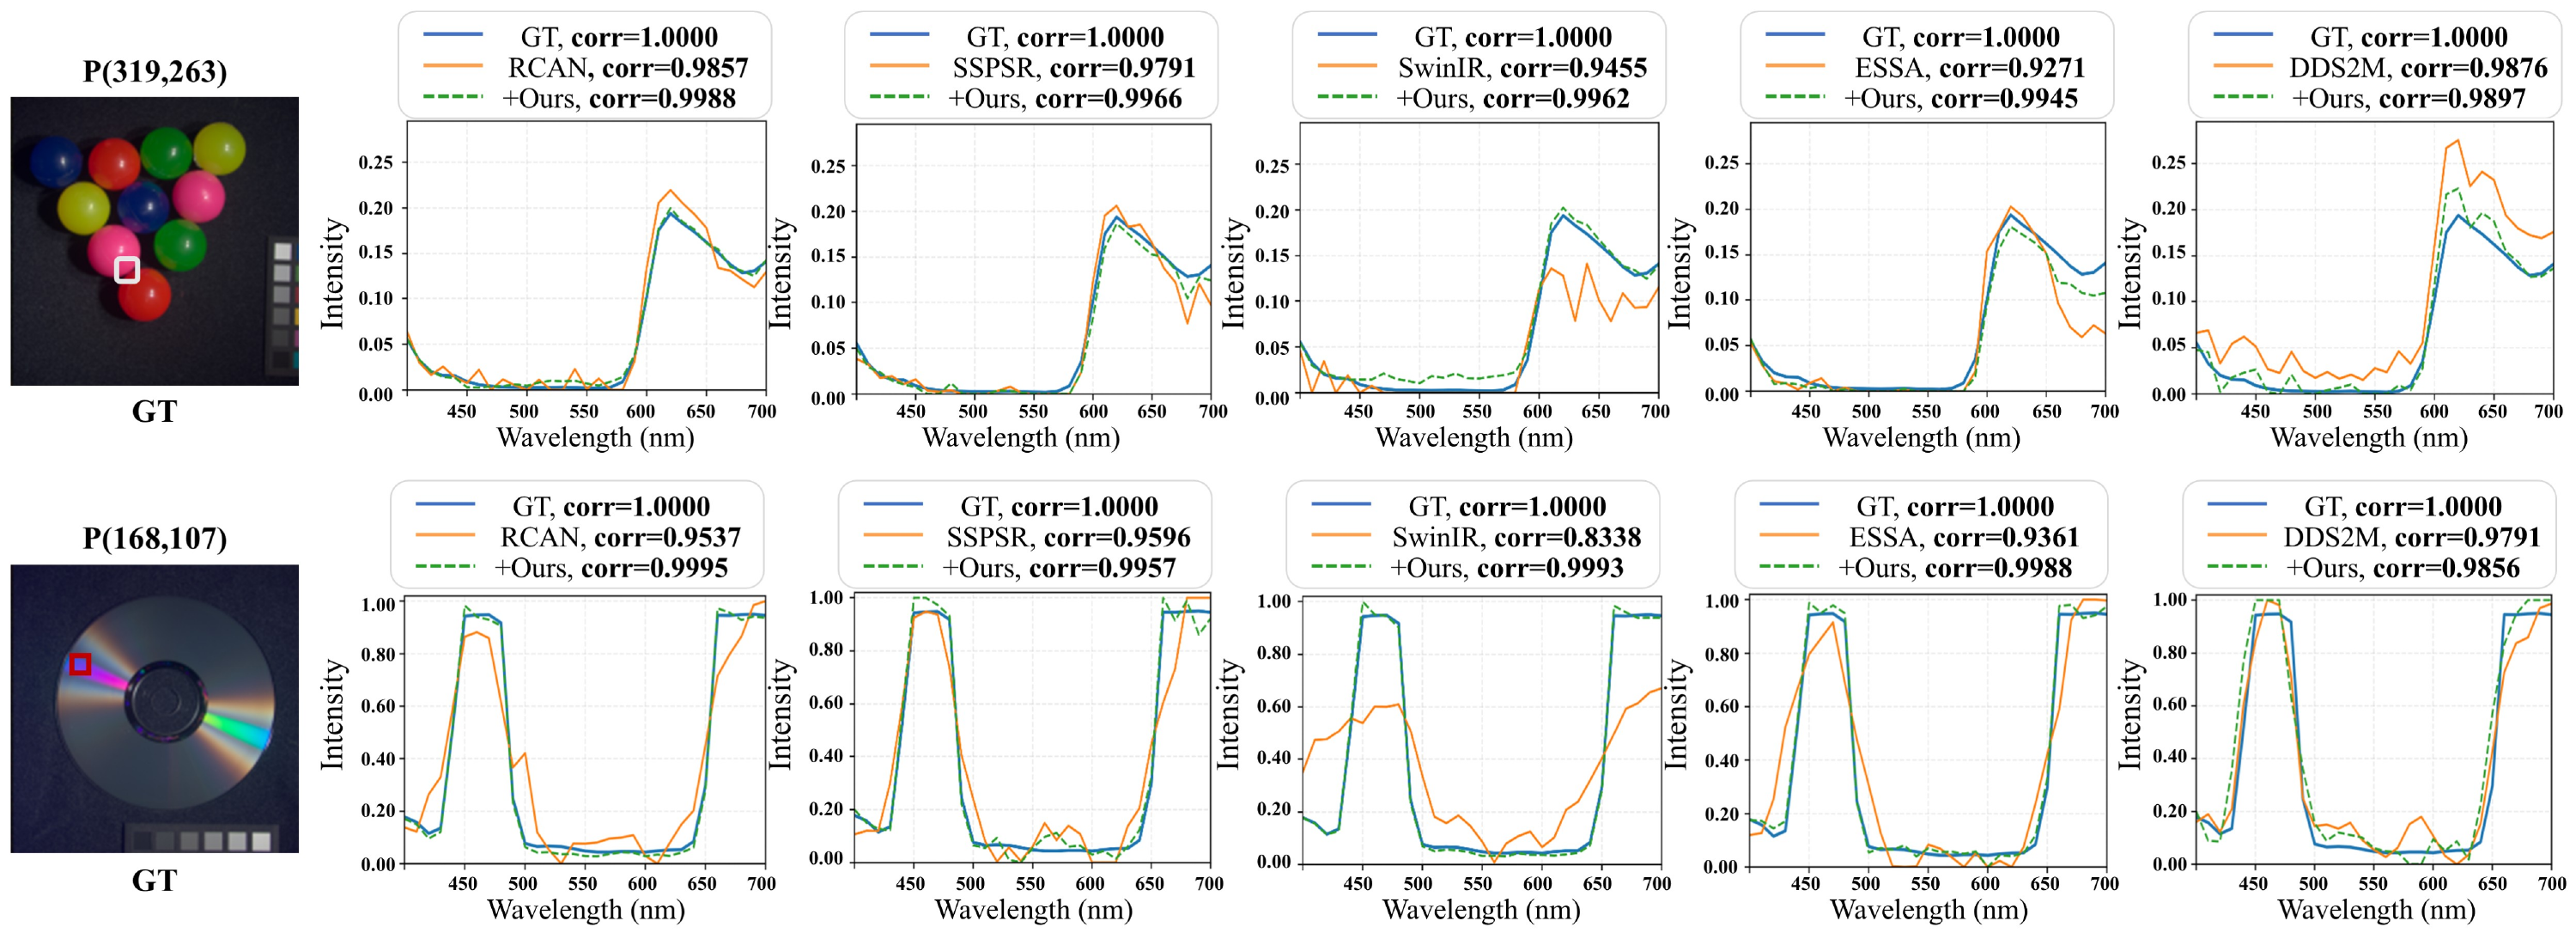}\vspace{2pt}
\includegraphics[width=\linewidth,height=0.285\textheight,keepaspectratio]{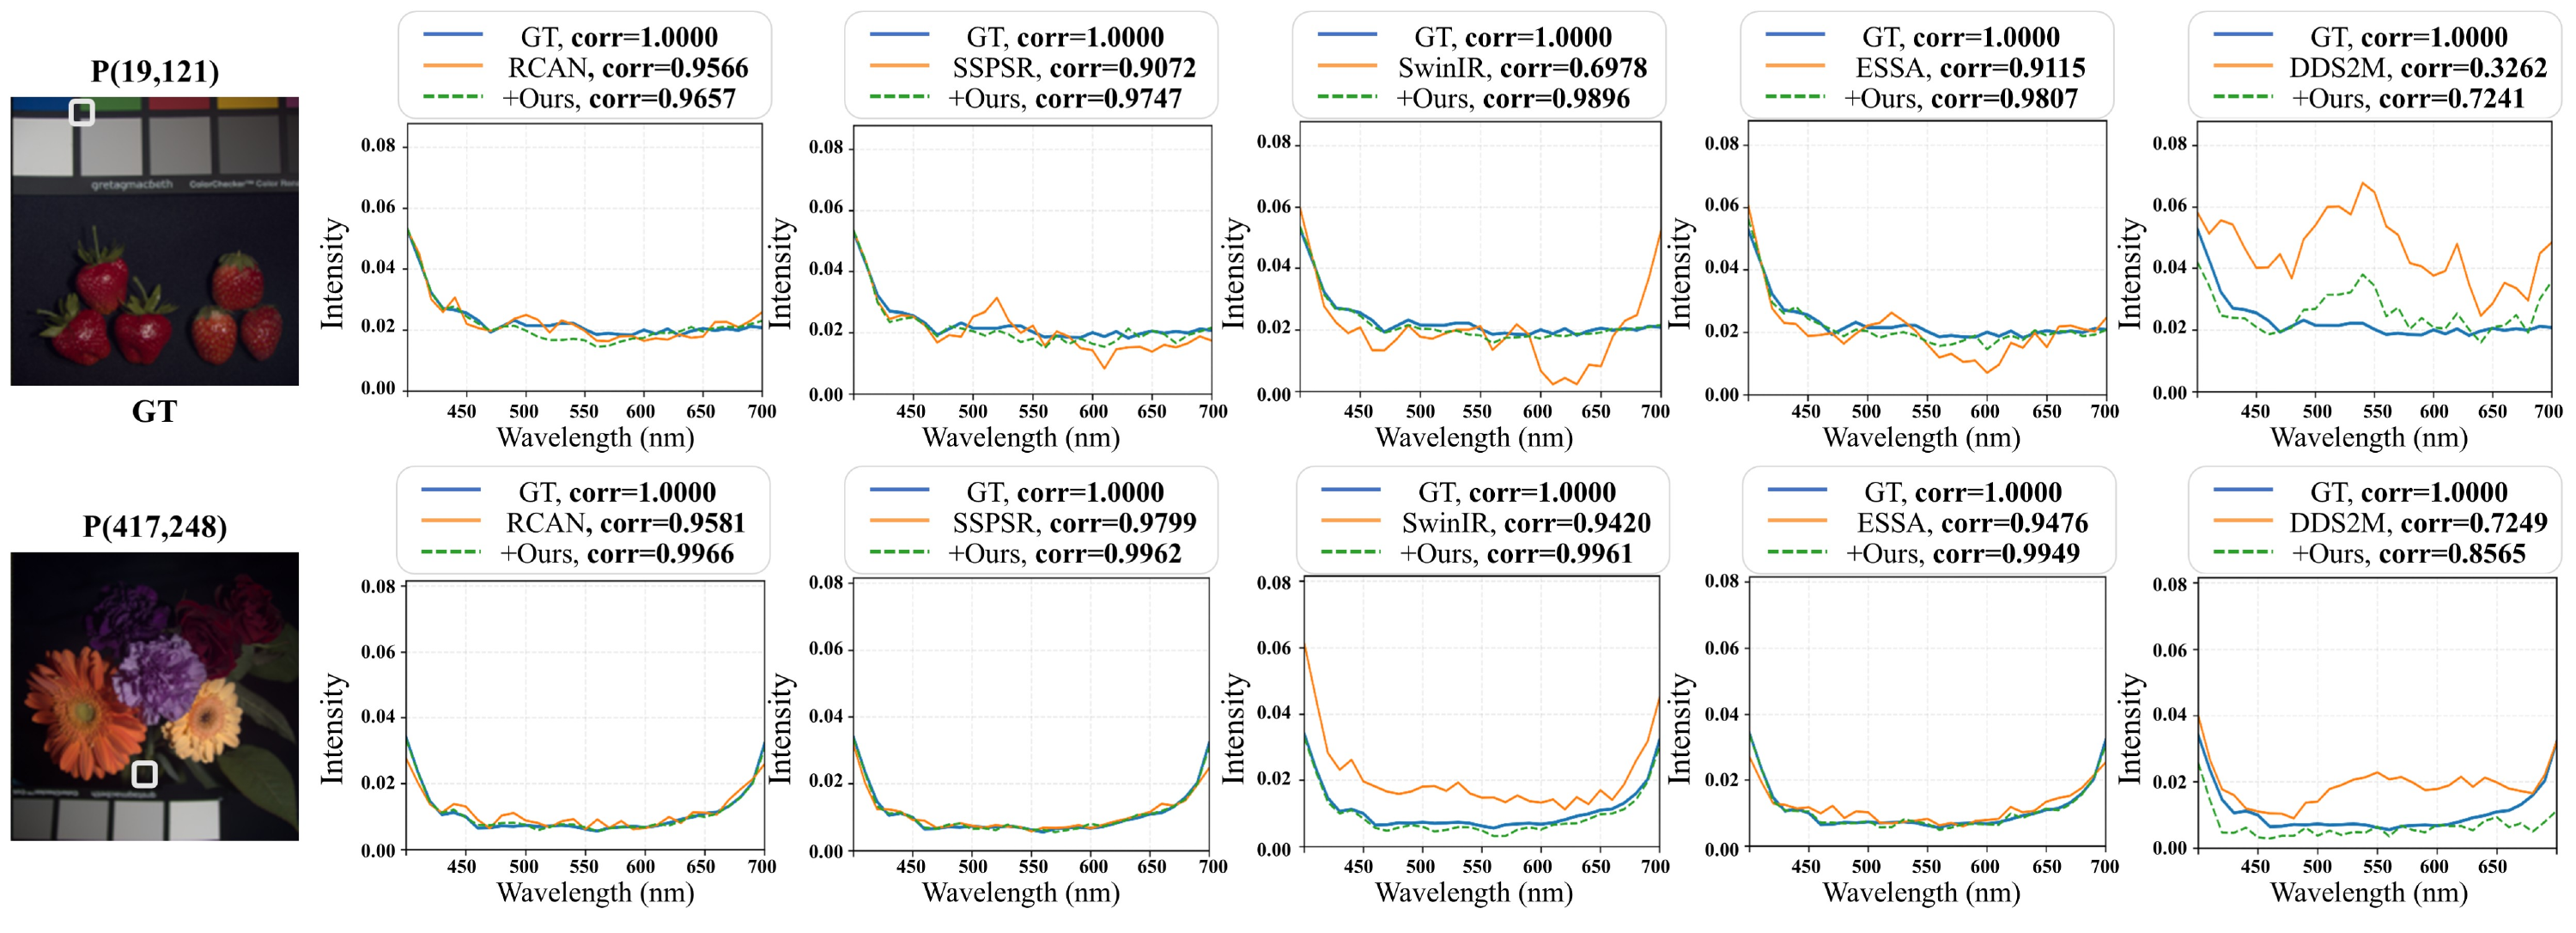}\vspace{2pt}
\includegraphics[width=\linewidth,height=0.285\textheight,keepaspectratio]{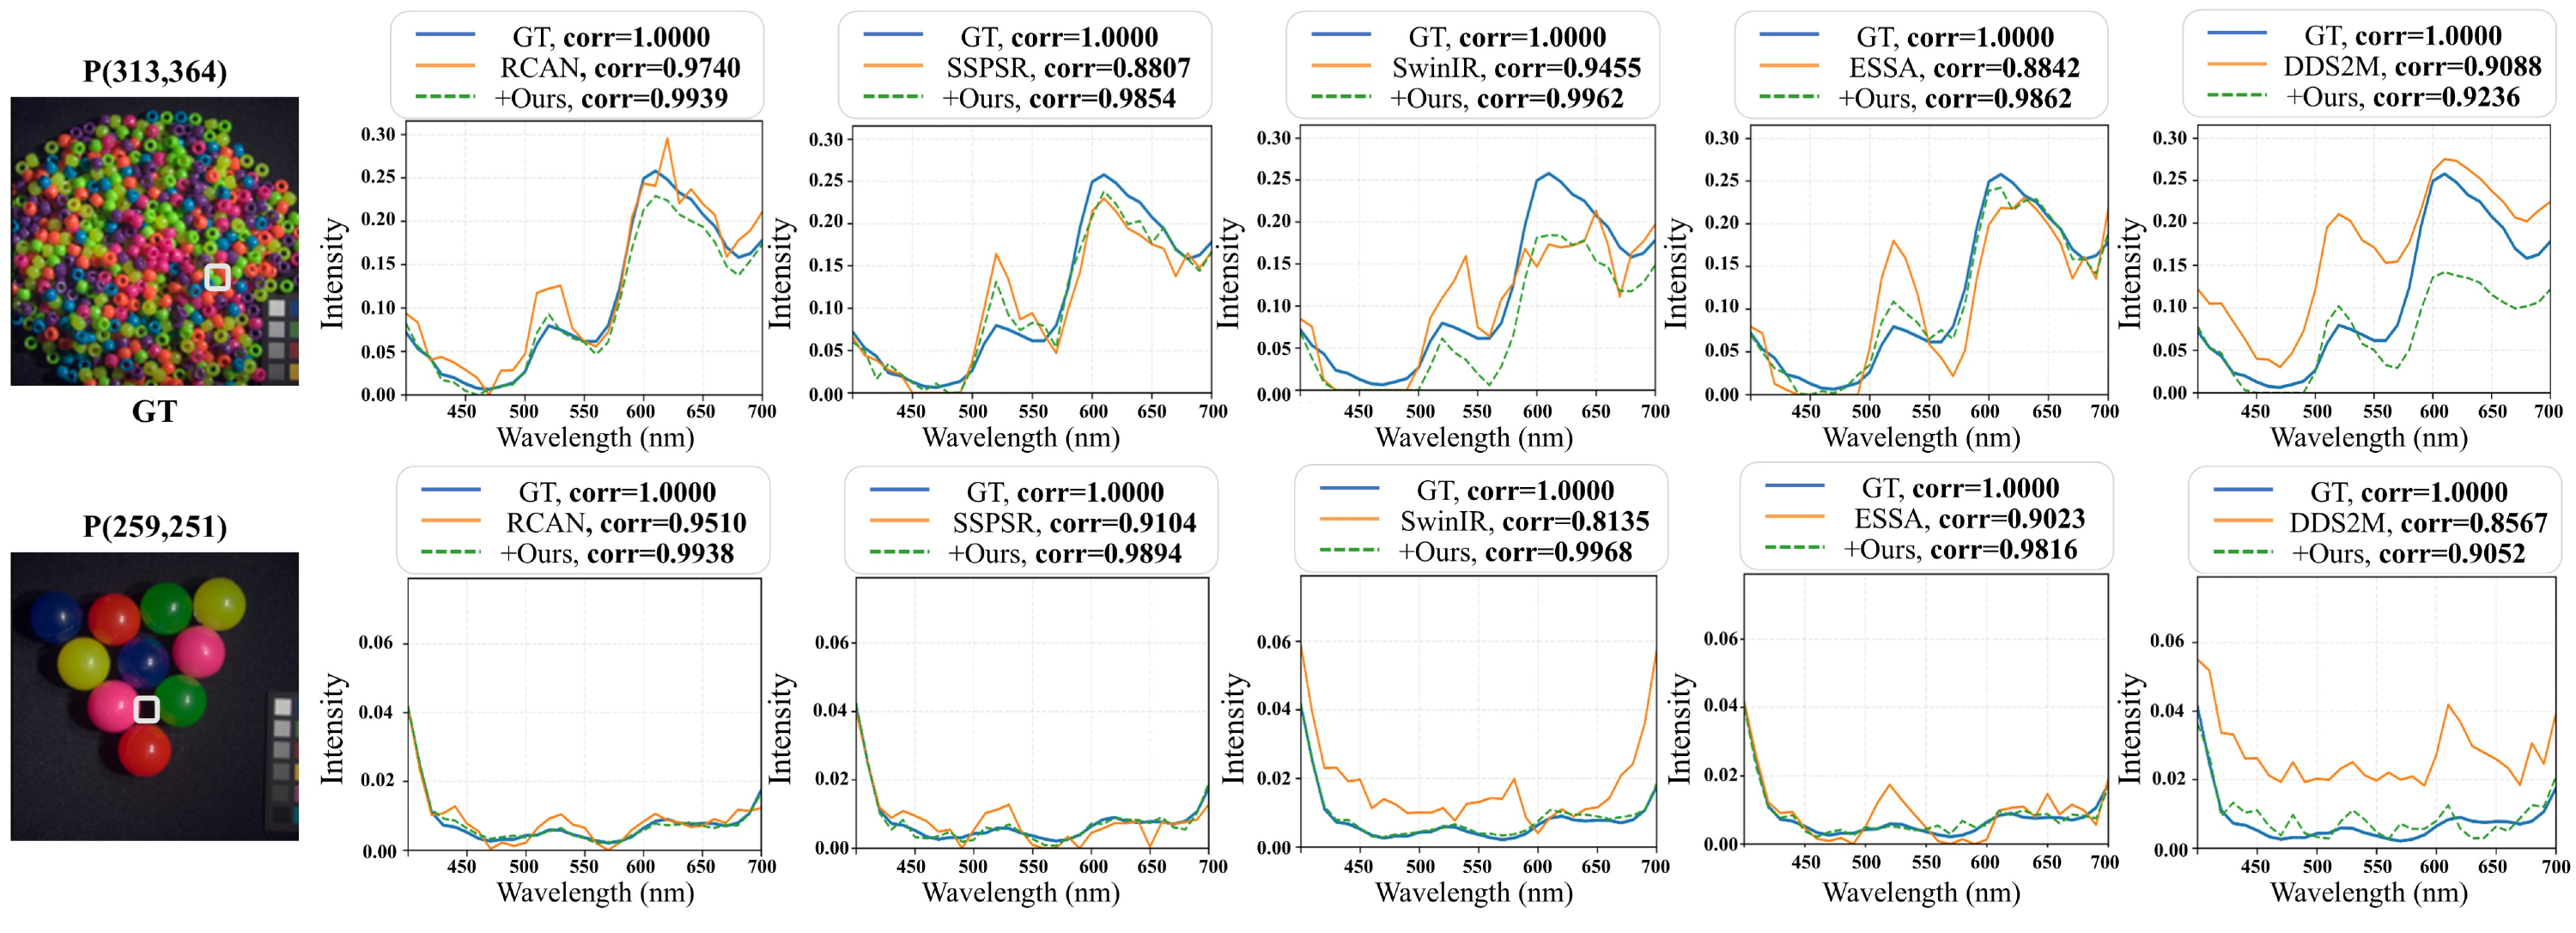}

\caption{Additional spectral curve gallery on CAVE at $\times4$.}
\label{fig:sp_cave_gallery}
\end{figure}

\FloatBarrier

% ---------- ICVL: 3 PDFs in one page ----------
\begin{figure}[!p]
\centering
\includegraphics[width=\linewidth,height=0.305\textheight,keepaspectratio]{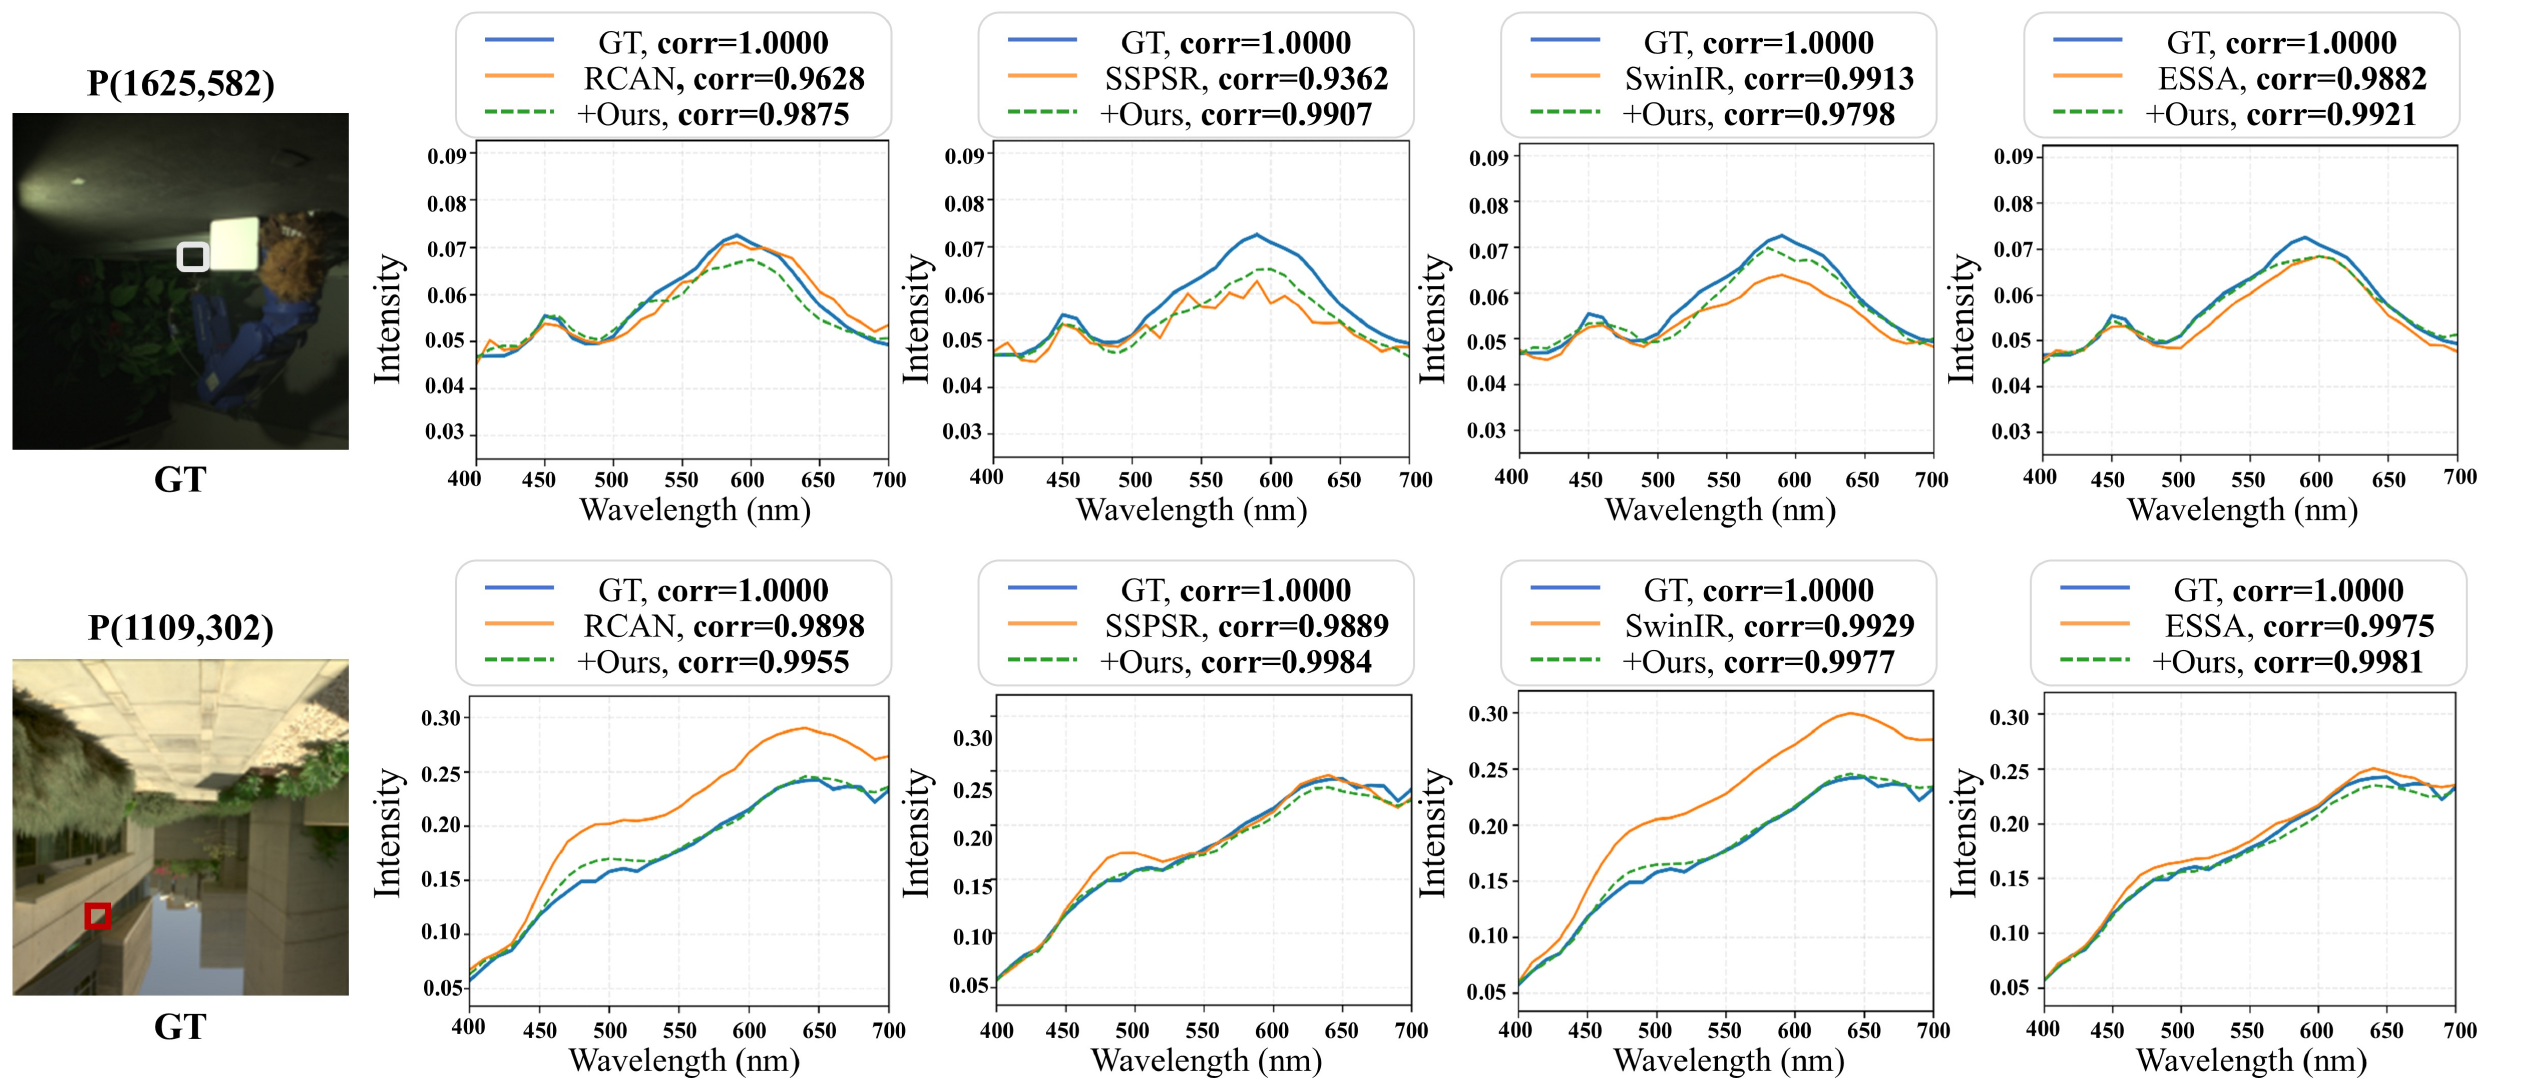}\vspace{2pt}
\includegraphics[width=\linewidth,height=0.305\textheight,keepaspectratio]{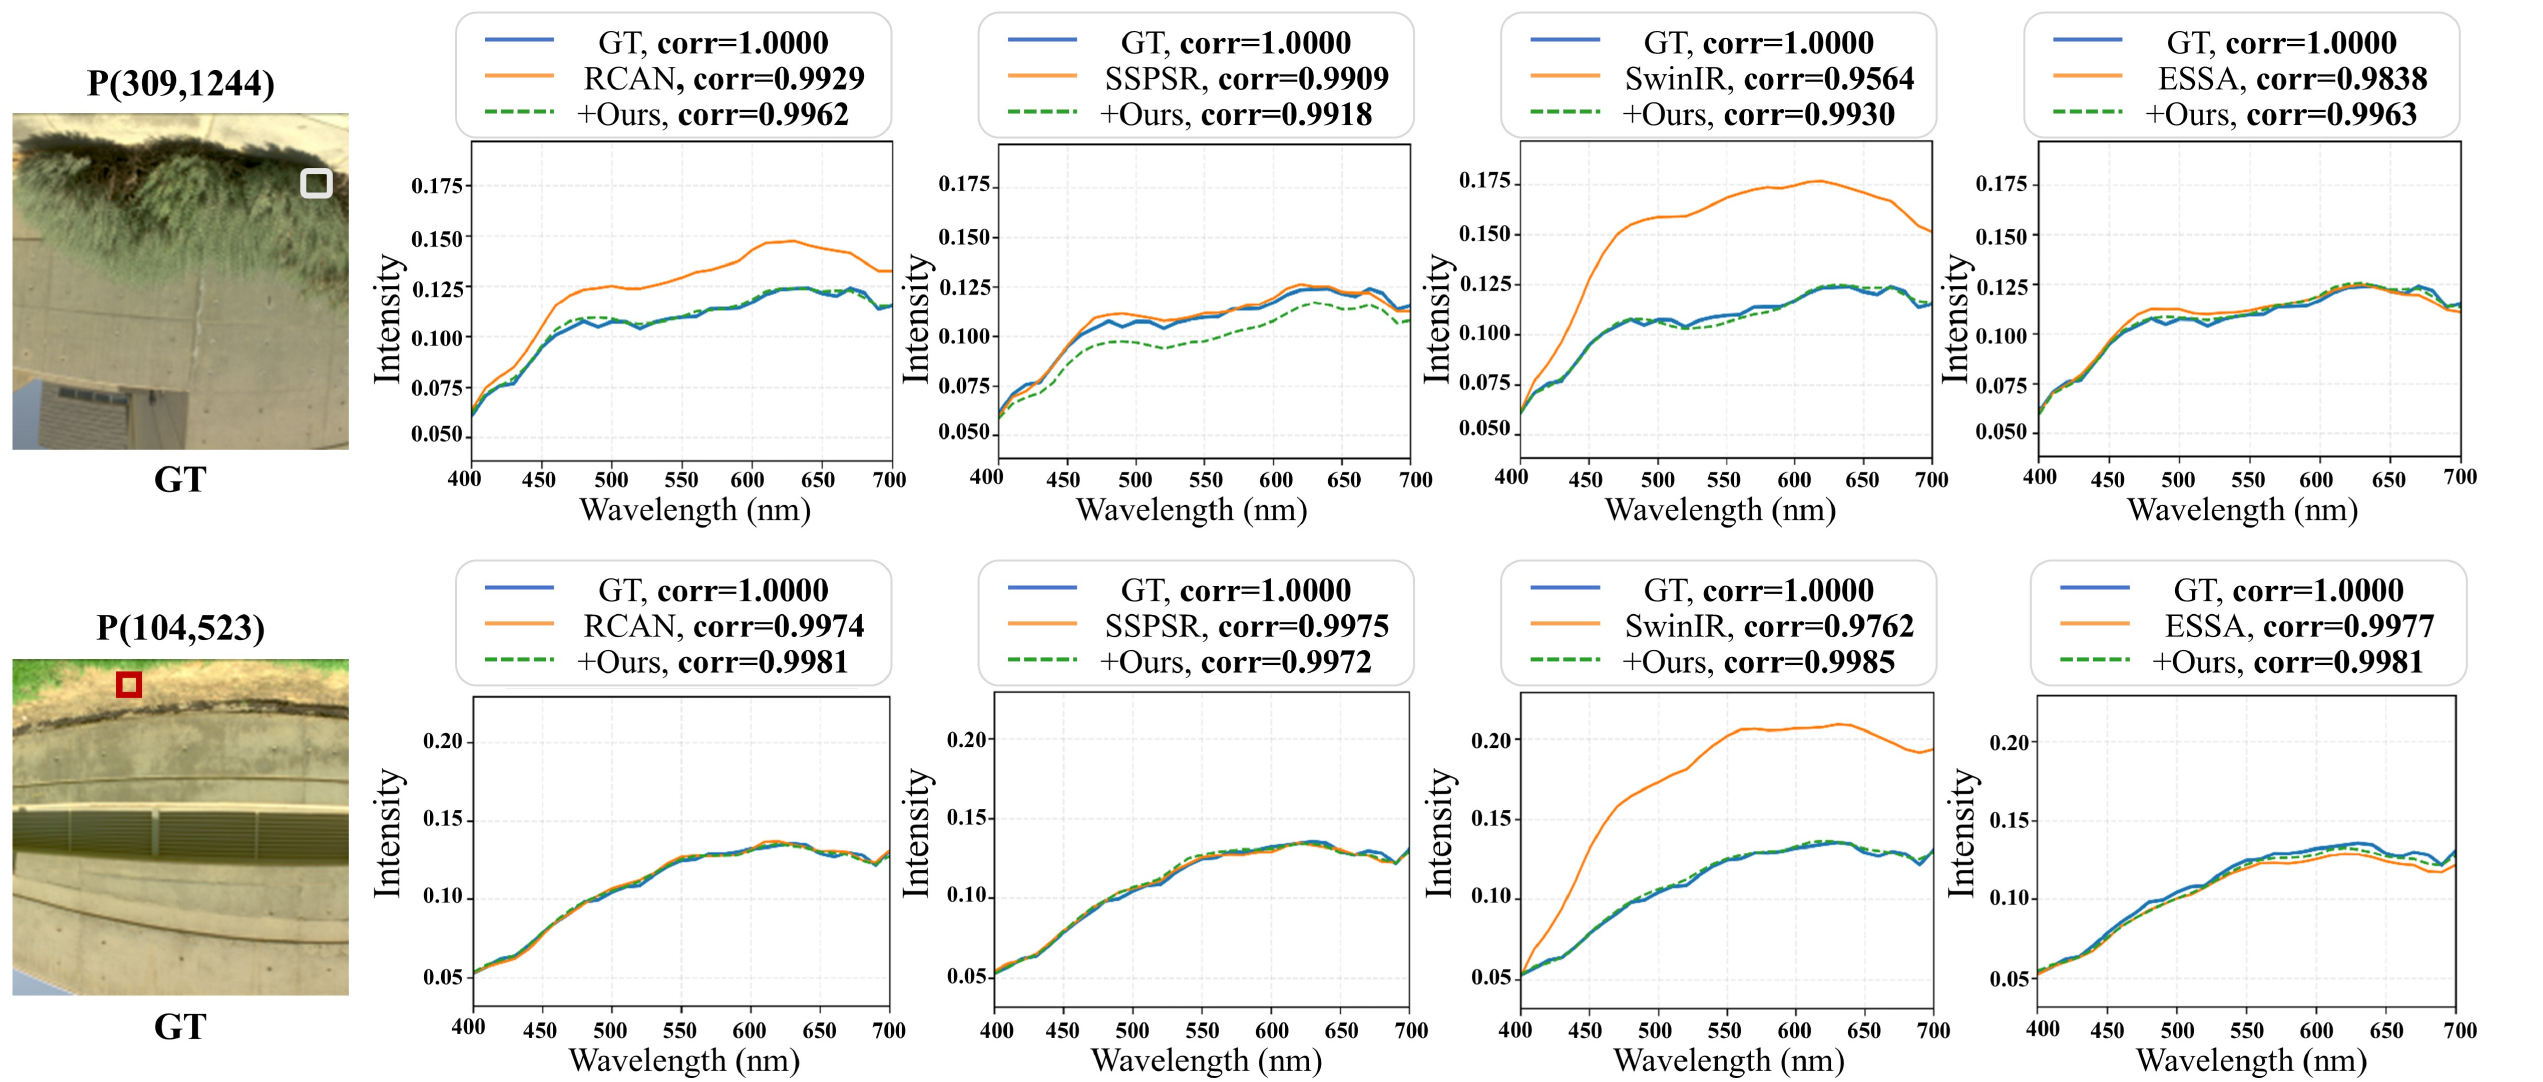}\vspace{2pt}
\includegraphics[width=\linewidth,height=0.305\textheight,keepaspectratio]{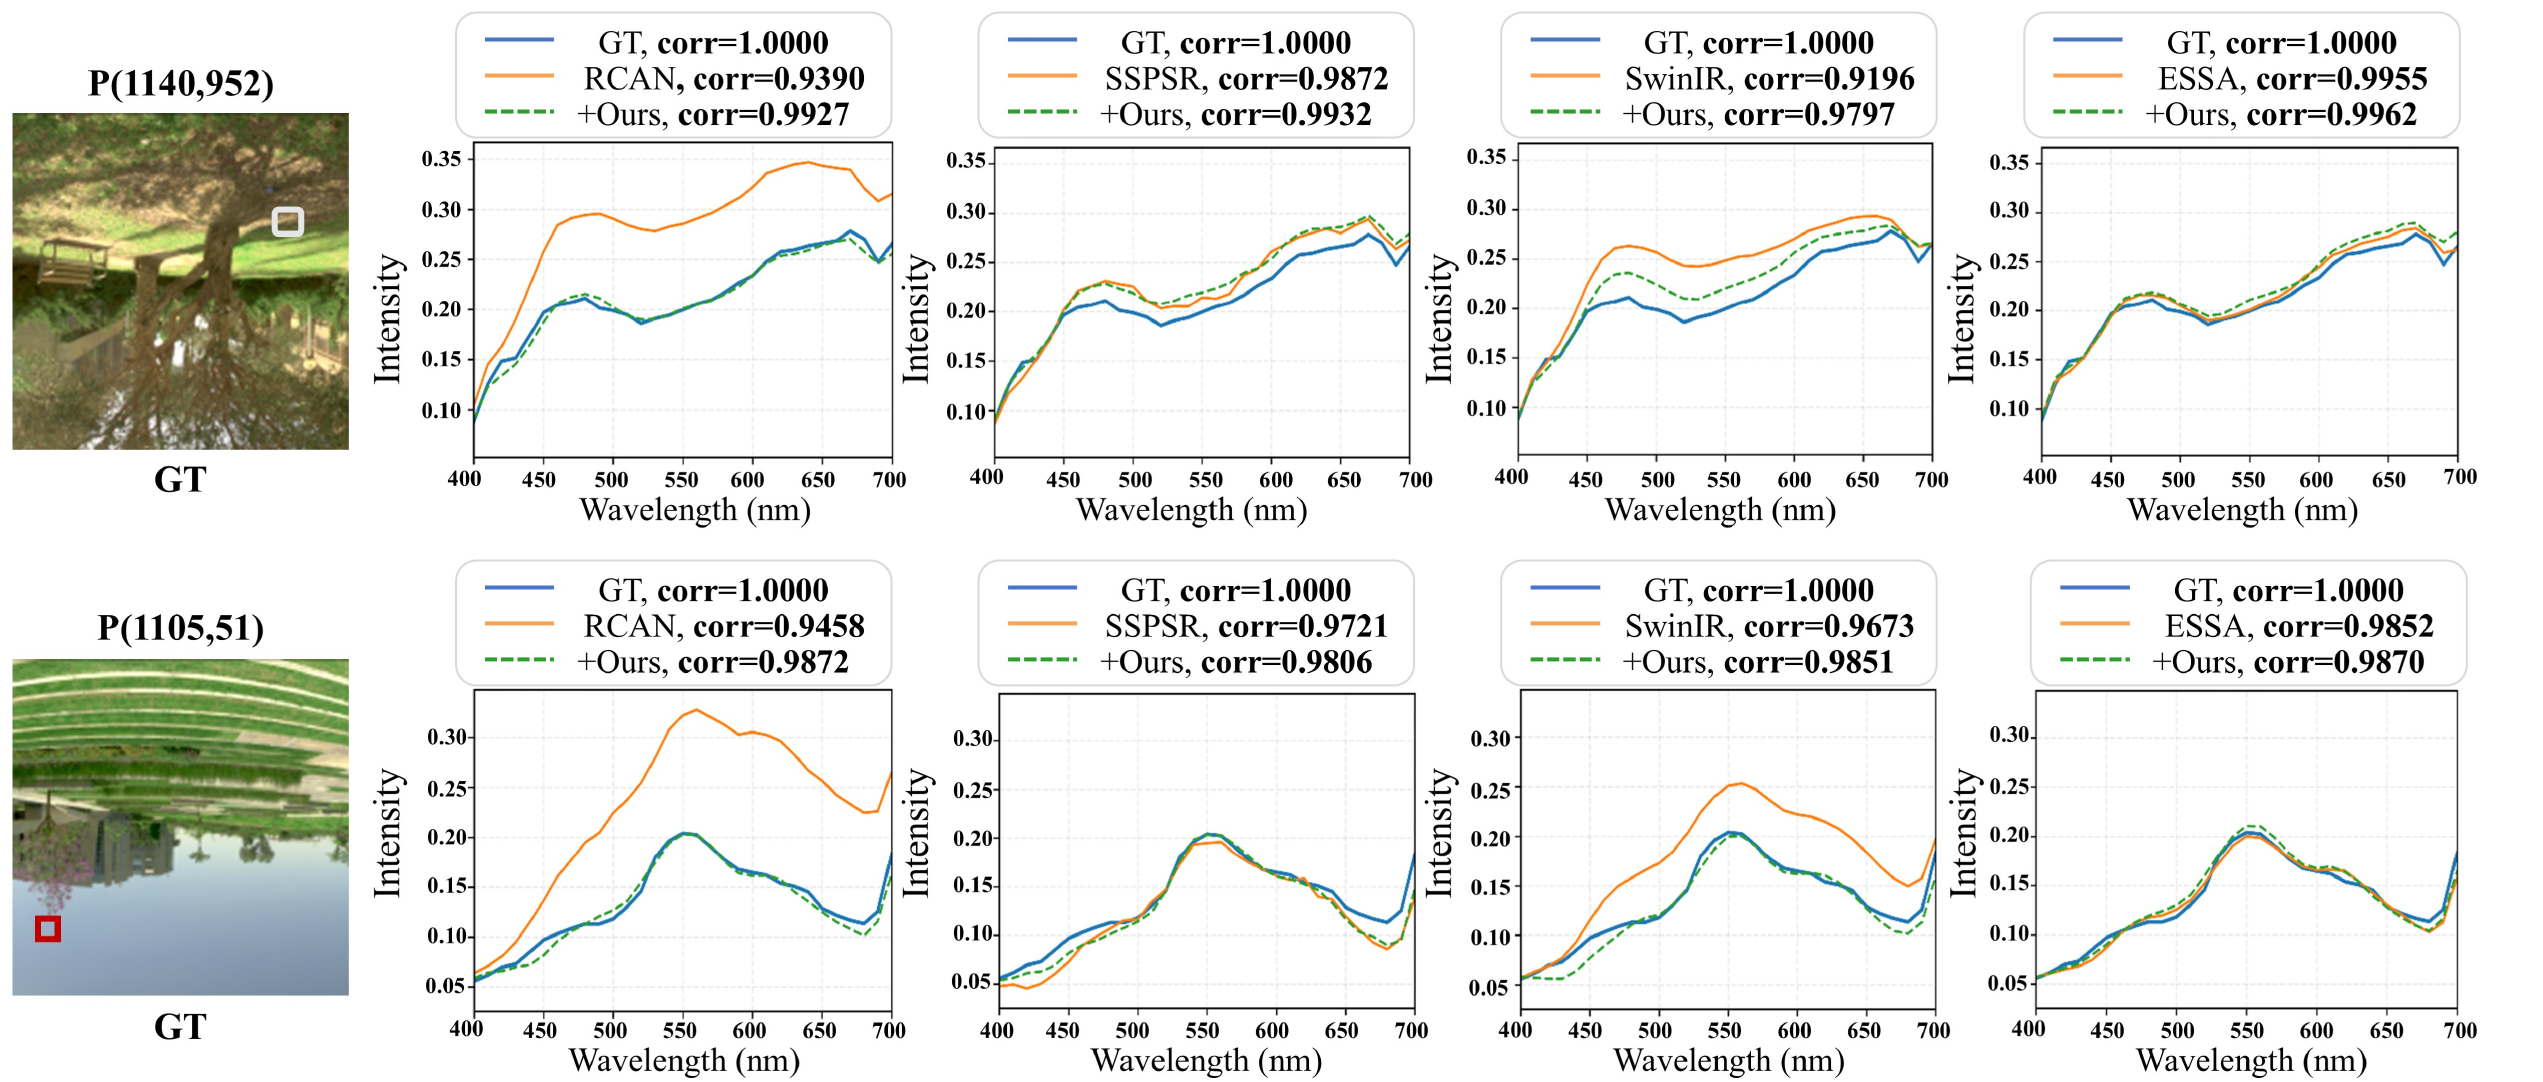}

\caption{Additional spectral curve gallery on ICVL at $\times4$. }
\label{fig:sp_icvl_gallery}
\end{figure}
\FloatBarrier

\subsection{Comparison to Simple Spectral Rectifiers}
To address the concern that spectral rectification might be achievable by simpler low-cost alternatives,
we compare~\name against three representative post-hoc spectral rectifiers.
All baselines operate on the output of a \emph{fixed} SwinIR model and do not modify the SR backbone weights.
In contrast,~\name is trained end-to-end as a plug-and-play rectification module.

\paragraph{Implementation details of SG/PCA/IBP.}
\textbf{Savitzky--Golay smoothing (SG).}
We apply a 1D Savitzky--Golay filter along the spectral dimension for each pixel independently.
We use a window length $w=7$ and polynomial order $p=3$.
To avoid boundary bias, the spectrum is symmetrically padded by reflection before filtering, and then cropped back to the original length.

\textbf{PCA projection.}
We fit a dataset-level PCA subspace using randomly sampled pixel spectra from the ARAD-1K training split and keep it fixed at test time.
We set the rank to $k=8$ and use $20{,}000$ sampled spectra in total.
Given an estimated spectrum, PCA rectification is performed by projection onto the top-$k$ principal components and reconstruction back to the original spectral space.

\textbf{Iterative back-projection (IBP).}
Starting from the SwinIR output, IBP refines the SR estimate by enforcing consistency with the observed LR image under an assumed degradation.
We perform $T=10$ refinement steps with step size $\eta=1.0$:
\begin{equation}
\textit{I}_{\mathrm{SR}}^{(t+1)}
=
\textit{I}_{\mathrm{SR}}^{(t)}
+
\eta \cdot \mathcal{U}
\!\left(
\textit{I}_{\mathrm{LR}}
-
\mathcal{D}\!\left(\textit{I}_{\mathrm{SR}}^{(t)}\right)
\right),
\end{equation}
where $\mathcal{D}$ is the same bicubic downsampling operator used in training and $\mathcal{U}$ is its corresponding bicubic upsampling.
IBP is applied independently to each spectral band, which keeps the procedure lightweight while improving degradation consistency.

\paragraph{Quantitative comparison on ARAD-1K.}
Tab.~\ref{tab:app_simple_rectifiers} reports results on ARAD-1K with SwinIR as the base SR model.
SG can suppress oscillations but often over-smooths informative spectral variations, leading to worse reconstruction.
PCA projection imposes a low-rank spectral prior and improves spectral fidelity over SG, but its gain is limited by a fixed subspace and weak spatial adaptivity.
IBP improves measurement consistency, yet it cannot directly correct cross-band structural errors from the backbone, resulting in smaller improvements in spectral metrics and MCR.

Compared with these low-cost alternatives,~\name achieves the best overall performance across all scales, improving spatial quality and spectral fidelity while also yielding the highest MCR.
This suggests that effective rectification requires more than smoothing or a global low-rank prior, and benefits from content-adaptive cross-band correction coupled with spatial structures.
For clarity, we report~\name as an additional row in Tab.~\ref{tab:app_simple_rectifiers}.
\name is trained end-to-end, whereas SG/PCA/IBP are post-hoc operations applied to a fixed SwinIR output.
